# Supplementary material for: A Generalized Theory for Optical Cooling of a Trapped Atom with Spin
Source: arXiv:2406.19153 source file (2024-09-19)
Supplement: Supplementary file 1 [file SM.tex]

% \documentclass[%
% preprint,
% %reprint,
% %superscriptaddress,
% %groupedaddress,
% %unsortedaddress,
% %runinaddress,
% %frontmatterverbose, 
% %preprintnumbers,
% %nofootinbib,
% %nobibnotes,
% %bibnotes,
%  amsmath,amssymb,
% %aps,
% pra,
% %prb,
% %rmp,
% %prstab,
% %prstper,
% %floatfix,
% ]{revtex4-2}
% \usepackage{subcaption}
% \usepackage{graphicx}% Include figure files
% \usepackage{wrapfig}
% \graphicspath{ {./images/} }
% \usepackage [english]{babel}
% \usepackage [autostyle, english = american]{csquotes}
% \MakeOuterQuote{"}
% \usepackage{dcolumn}% Align table columns on decimal point
% \usepackage{bm}% bold math
% \usepackage{hyperref}% add hypertext capabilities
% \usepackage{soul}
% %\usepackage[mathlines]{lineno}% Enable numbering of text and display math
% %\linenumbers\relax % Commence numbering lines
% %\usepackage{xcolor}
% \usepackage[dvipsnames]{xcolor}
% \newcommand{\Jon}[1]{\textcolor{blue}{#1}}
% \newcommand{\Karl}[1]{\textcolor{ForestGreen}{#1}}
% \newcommand{\Saumitra}[1]{\textcolor{purple}{#1}}
% \newcommand{\delete}[1]{\textcolor{red}{#1}}
% %\usepackage[showframe,%Uncomment any one of the following lines to test 
% %%scale=0.7, marginratio={1:1, 2:3}, ignoreall,% default settings
% %%text={7in,10in},centering,
% %%margin=1.5in,
% %%total={6.5in,8.75in}, top=1.2in, left=0.9in, includefoot,
% %%height=10in,a5paper,hmargin={3cm,0.8in},
% %]{geometry}

% \begin{document}

% %\preprint{APS/123-QED}

% \title{SM}% Force line breaks with \\

% \author{Saumitra Phatak}
%  %\altaffiliation[Also at ]{Physics Department, XYZ University.}%Lines break automatically or can be forced with \\
% \author{Karl Blodgett}
% \author{David Peana}
% \author{Jonathan Hood (author order random)}%
%  %\email{Second.Author@institution.edu}
% %\affiliation{%
% %Authors' institution and/or address \\
% %}%

% \date{\today}% It is always \today, today, but any date may be explicitly specified


% \maketitle

% % and the the ground-state collapse operator in the large detuning limit is
% % \begin{gather} 
% % L^\text{eff}_{q,\pm} = - \frac{\Omega}{2} \left[  \frac{ ( e^{\pm ik\hat{x}} \bm{e}_q^* \cdot \bm{D}) (\bm{\epsilon}(\hat{x}) \cdot \bm{D}^\dag) }{ \Delta - i \Gamma/2}   \right].
% % \end{gather}

% % \begin{equation}
% %     \tan{\theta} = \Omega_2/\Omega_1,
% % \end{equation}
% % \begin{equation}
% %     \cos \theta = \Omega_1/ \Omega_{\text{rms}}^2 \quad  \sin \theta = \Omega_2/ \Omega_{\text{rms}}^2
% % \end{equation}
% % 
% % \begin{gather}
% % |g_{\scriptscriptstyle B}\rangle = \cos{\theta} \, |g_1 \rangle + \sin{\theta} \, |g_2 \rangle \nonumber   \\
% % |g_{\scriptscriptstyle D}\rangle = - \sin{\theta} \, |g_1 \rangle + \cos{\theta} \, |g_2 \rangle \\
% % |e \rangle = |e \rangle.
% % \end{gather}

% % \begin{gather}
% % \Delta_{\scriptscriptstyle B} = \cos^2{ \theta } \,\, \Delta_1 +  \sin^2{ \theta } \,\, \Delta_2  \nonumber \\
% % \Delta_{\scriptscriptstyle D} = \sin^2{ \theta } \,\,\Delta_1 +  \cos^2{ \theta }\,\, \Delta_2,
% % \end{gather}

% % The transformed collapse operators are 
% % \begin{gather}
% %     L_{B,\pm} =  \sqrt{\Gamma} \,\, e^{\pm ik\hat{x}} \left(\sin{\theta} \, \hat{D}_{B} + \cos{\theta} \,  \hat{D}_{D}  \right)  \\
% %       L_{D,\pm} =  \sqrt{\Gamma} \,\, e^{\pm ik\hat{x}} \left(\cos{\theta} \, \hat{D}_{B} - \sin{\theta} \,  \hat{D}_{D}  \right).
% % \end{gather}


% % In the bright and dark basis, 
% % \begin{gather}
% %     H_\text{eff} =   \frac{|\Omega_B|^2 |g_{\scriptscriptstyle B} \rangle \langle g_{\scriptscriptstyle B}| + |\Omega_D|^2 |g_{\scriptscriptstyle D} \rangle \langle g_{\scriptscriptstyle D}| +  \right. \\ 
% %     \left. ( \Omega_B^* \Omega_D |g_{\scriptscriptstyle B} \rangle \langle g_{\scriptscriptstyle D}| + h.c.  ) 
% %      \right]
% % \end{gather}
% % where $\Omega_B = \Omega_1 \cos(\theta) e^{ik_1 \hat{x}} + \Omega_2 \sin\theta e^{i k_2 \hat{x}} $   and $\Omega_D = -\Omega_1 \sin\theta e^{ik_1 \hat{x}} + \Omega_2 \cos\theta e^{i k_2 \hat{x}} $ .
% % When $k_2 = - k_1 = k$ and $\Omega_1 = \Omega_2$,  then   $\Omega_B = 2 \Omega \cos( k\hat{x})$  and $\Omega_D = 2 \Omega \cos(k\hat{x})$.     Then the effective Hamiltonian is 
% % % \frac{\Delta}{\Delta^2 + \Gamma^2/4} 
% % See brightdark.nb for these derivations in dropbox.


% % first order in the LD parameter, which gives \Jon{shouldn't you get k1-k2}
% % \begin{gather}
% %     H_I = \Omega_{\scriptscriptstyle \text{\text{rms}}} \, D_{\scriptscriptstyle B}  +  i k \hat{x} \, \frac{ 2 \Omega_1 \Omega_2}{\Omega_\text{\text{rms}}} \, D_{\scriptscriptstyle D}   + h.c.  ,
% %     %+ i k \hat{x} \frac{\Omega_1^2 - \Omega_2^2}{\Omega_\text{rms} } \, D_{B} 
% % \end{gather}
% % where $ \Omega_\text{rms} = \sqrt{ \Omega_1^2 + \Omega_2^2} $. The first term only drives the bright states, resulting optical pumping out of the bright state and a bright state light shift. The position dependent term, which is 1st order in the LD parameter, drives the dark state to $n \pm 1$.


% % The 0th order term results in a light shift for just a bright state.  The population is pumped to a dark the state.  The criteria for cooling is the pumped state much be lower in energy.  Consequently, this scheme only works in the blue-detuned case, where the bright state is shifted to higher energy.  



% %In the limit of large detuning, all rates go to zero except for $\Gamma_R$, which then gives that $P_{\up}(n+1) = P_{\down}(n)$.  The population is in equilibrium between these two states.  

% % An expression for the ratio of population between neighboring motional states
% % \begin{equation}
% % \frac{P(n+1)}{P(n)} = \frac{\gamma_r \eta^2 + ( \eta^2 \gamma_r + \gamma_{\scriptscriptstyle +} ) \frac{\Omega_R^2}{\gamma_r^2} }{ \gamma_s \eta^2 + ( \eta^2 \gamma_s + \gamma_{\scriptscriptstyle -} ) \frac{\Omega_R^2}{\gamma_r^2} }.
% % \end{equation}
% % This is the final result of this model.
  
% %\[\frac{P(n+1)}{P(n)} = \exp{(-\hbar \nu / k_B T) }.\]
% %If the ratio is $s$, the the normalized solution is $P(n) = (1-s) s^n$. Then the final energy is $\langle n\rangle = \frac{s}{1-s}$.
% % Because $\Omega_R$ scales as $1/\Delta$ and $\gamma_R$ scales as $1/\Delta^2$, the ratio $(\Omega_R/ \gamma_R)^2$ scales as $\Delta^2$ and becomes dominant in the limit of large detuning. 


% % First, we rewrite the two scalar products as the scalar product of two rank 2 matrices:
% % \begin{equation}
% %  (\bm{A}^* \cdot \hat{\bm{D}} ) (\hat{\bm{D}}^\dag  \cdot \bm{B}) =  (\bm{A}^* \otimes \bm{B}) \cdot (\hat{\bm{D}} \otimes \hat{\bm{D}}^\dag)  
% % \end{equation}
% % A rank 2 tensor or matrix can always be decomposed into three parts: a rank 0 part that does not change upon rotation, a rank 1 part that rotate as a vector, and a rank 2 part that rotates as a tensor.  In Cartesian or spherical basis, the scalar product above can be decomposed into a sum of scalar products of each rank:
% % \begin{equation}
% %     \sum_k   (\bm{A}^* \otimes \bm{B})^{(k)} \cdot (\bm{D} \otimes \bm{D}^\dag )^{(k)}
% % \end{equation}
% % The term $(\bm{D} \otimes \bm{D}^\dag )^{(k)}$ is a rank $k$ vector operator in the ground state spin basis $F$.   We will now use the spherical vector basis so that we can apply the Wigner-Eckert theorem.  The Wigner-Eckert theorem tells us that any rank $k$ can be expressed in terms of a Clebsch-Gordon coefficient times a reduced matrix element.    We then obtain the identity~\cite{}:
% % \begin{gather} \label{eq:scalaridentity}
% %   (\bm{A}^* \!\cdot\! \hat{\bm{D}})( \hat{\bm{D}}^\dag \!\cdot\! \bm{B}) =  \nonumber \\
% %      C^{(0)}  (\bm{A}^* \!\cdot\! \bm{B}) %\nonumber \\
% %     + i C^{(1)} (\bm{A}^* \! \times \! \bm{B}) \cdot \hat{\bm{F}} + \nonumber \\
% %       C^{(2)} \left(  \frac{ (\bm{A} \! \cdot \! \hat{\bm{F}})^\dag (\bm{B} \!\cdot\! \hat{\bm{F}}) + (\bm{A}\! \cdot \! \hat{\bm{F}}) (\bm{B} \! \cdot \! \hat{\bm{F}})^\dag}{2}   - \frac{1}{3} \hat{\bm{F}}^2 (\bm{A}^* \! \cdot \! \bm{B}) \right) 
% % \end{gather}

% % This can be seen for example as $(a_i \hat{D}_i) (\hat{D}^\dag_j b_j) =  (a_i b_j) (\hat{D}_i \hat{D}^\dag_j) $.

% % This is the scalar product of two rank 2 matrices.  Both rank 2 matrices can either be represented in the cartesian or spherical vector basis.  In both basis, they can be separated into a rank 0, 1, and 2 parts.  THe rank 0 part does not change under rotation. THe rank 1 part rotates like a vector. The rank 2 part rotates likes a rank 2 matrix. 
% % The scalar product can then be separated into each part 

% % Vectors are expressed in the spherical vector basis with $V_0 = V_z$, $V_{\pm 1} = \mp (V_x - i V_y)/\sqrt{2}$.  
% %For example, the dipole operator can be expresed in terms of the spherical basis unit vectors as 
% % \begin{equation}
% % \bm{d} = \sum_q d_q \hat{\bm{e}}_q^*,
% % \end{equation}
% %with components $d_{\pm1} = \mp \frac{1}{\sqrt{2}} (d_x \pm i d_y)$ and $d_0 = d_z$. 
% % The spherical vectors have the following useful the properties.  The complex conjugate of a component is  $(d_q)^* = (-1)^q d_{-q}$.  The dots product between two spherical vectors is $\bm{A} \cdot \bm{b} = \sum_q (-1)^q a_q b_{-q} = \sum_q a_q b_q^*$.  The orthogonality of two basis vectors is shown by  $\hat{e}_q \cdot \hat{e}_{q'}^* = \delta_{qq'}$.

% % \begin{equation}
% %     \sum_k   (\bm{a}^* \otimes \bm{b})^{(k)} \cdot (\bm{D} \otimes \bm{D}^\dag )^{(k)}
% % \end{equation}
% % The term $(\bm{D} \otimes \bm{D}^\dag )^{(k)}$ is a rank $k$ vector operator in the ground state spin basis $F$.   We will now use the spherical vector basis so taht we can apply the Wigner-Ecker theorem.  The Wigner-Eckert theorem tells us that any rank $k$ can be expressed in terms of a Clebsch-Grodon coefficient times a reduced matrix elelemtn.   
% % %
% % \begin{gather} 
% %     (\bm{D} \otimes \bm{D}^\dag )^{(0)}_0  \propto 1  \\
% %     (\bm{D} \otimes \bm{D}^\dag )^{(1)}_q  \propto F_q  \\
% %     (\bm{D} \otimes \bm{D}^\dag )^{(2)}_q  \propto  \{ \bm{F} \otimes \bm{F} \}^{(2)}_q  
% % \end{gather}
% % %
% % \begin{equation}
% %     \langle m_F |  (\bm{D} \otimes \bm{D}^\dag )^{(k)}_q   | m'_F \rangle =  \langle F || (\bm{D} \otimes \bm{D}^\dag )^{(k)} || F \rangle \,\, \langle  F m_F ; k q  | F m'_F  \rangle  
% % \end{equation}
% % But that implies that it is equivalent up to the reduced matrix element to any other rank $k$ within this spin space.   Rank 0 is just the identity,  Rank 1 can then be expressed in terms of the spin operator $F_q$,  and rank 2 in terms of the outer product $F \otimes F$. 

% % In the paper we use this and this. 
% % \begin{gather}
% %     H_A =\frac{\Omega^2}{4 \Delta} \left[  C^{(0)} |\bm{\epsilon}|^2 + i C^{(1)} (\bm{\epsilon}^* \times \bm{\epsilon}) \cdot \bm{F}  + C^{(2)} \left( \frac{1}{2} \left((\bm{\epsilon} \cdot \bm{F})^\dag (\bm{\epsilon} \cdot \bm{F}) + (\bm{\epsilon} \cdot \bm{F}) (\bm{\epsilon} \cdot \bm{F})^\dag \right)   - \frac{1}{3}\bm{F}^2 |\epsilon|^2 ) \right)  \right]
% % \end{gather}
% % \Jon{appendix}
% % \begin{gather}
% %     W_q = \frac{\Omega/2}{\Delta + i \Gamma/2} \left( C^{(0)} e_q \cdot \epsilon + i C^{(1)} (e_q \cdot \epsilon)\cdot F + C^{(2)} \left[ \frac{()() + ()()}{2} - 1/3 F^2 e_q \cdot \epsilon  \right] \right)
% % \end{gather}

% % ---------------------------------------------------
% % \[
% % \sum_{n=0}^{\infty} n \frac{dP_{-}(n)}{dt} = G \sum_{n=0}^{\infty} (n+1) P_{+}(n) - G \sum_{n=0}^{\infty} n (n+1) P_{-}(n) + \gamma_{-} \sum_{n=0}^{\infty} n P_{+}(n) - \gamma_{+} \sum_{n=0}^{\infty} n P_{-}(n) 
% % + \eta^2 \gamma_{-} \left[ \sum_{n=0}^{\infty} (2n^2 + 3n + 1) P_{+}(n) - \sum_{n=0}^{\infty} n (2n+1) P_{-}(n) \right]
% % \]


% % \[
% % \sum_{n=0}^{\infty} n \frac{dP_{+}(n)}{dt} = G \sum_{n=0}^{\infty} (n^2 - n) P_{-}(n) - G \sum_{n=0}^{\infty} n^2 P_{+}(n) - \gamma_{-} \sum_{n=0}^{\infty} n P_{+}(n) + \gamma_{+} \sum_{n=0}^{\infty} n P_{-}(n)
% % + \eta^2 \gamma_{+} \left[\sum_{n=0}^{\infty} (2n^2 + 3n + 1) P_{-}(n) - \sum_{n=0}^{\infty} n (2n+1) P_{+}(n)\right]
% % \]

% % \[
% % \sum_{n=0}^{\infty} n \left( \frac{dP_{-}(n)}{dt} + \frac{dP_{+}(n)}{dt} \right) = G \sum_{n=0}^{\infty} \left[ (1 - n^2) P_{+}(n) + (-n - n^2) P_{-}(n) \right]
% % + \eta^2 \sum_{n=0}^{\infty} \left[ \gamma_{-} (2n^2 + 3n + 1) P_{+}(n) + \gamma_{+} (2n^2 + 3n + 1) P_{-}(n) - \gamma_{-} n (2n+1) P_{-}(n) - \gamma_{+} n (2n+1) P_{+}(n) \right]
% % \]
% % --------------------------------------------


% %\tableofcontents
% % GM and EIT and $\Lambda-$GM have achieved  $P(n+1)/P(n) \approx \frac{\gamma_{\scriptscriptstyle +}}{\eta^2 \gamma_s} $.  Here $\gamma_{\scriptscriptstyle +}$ is the spontaneous emission that pumps to the dark state, and $\gamma_s$ is the scattering rate that leads to recoil.  Sub-doppler cooling for a bound atom requires 1) two spin states with different energy 2)  a  coupling between $n$ and $n-1$ of different spin states 2) optical pumping to the lower energy spin state.   We can overcome this limit by having a separate optical pumping beam with selection rules so that the dark state doesn't see it.  But why does EIT not do this. What is the fundmanetal limit to RSB then?  

 
% %  Don't typically use the bright and dark states of the the 3-level system. Instead relying on detuning so far that both are almost dark.  The spontaneous emission is incorporated by a third beam that uses selection rules to only pump g2 to g1.  For example by using 44 and 33 as g2 and g1, then using sigma plut to F=4 excited state, to which 44 is dark. and it decays to both states.

% % Use the ground state unrotated basis
% % \begin{equation}
% % H_0 = \Delta_1 |g_1 \rangle \langle g_1 | + \Delta_2 |g_1 \rangle \langle g_1 | + \nu a^\dag a
% % \end{equation}
% % We are currently assuming all three potentials have the same trapping frequency. We define two dipole operators 
% % Without spin, 
% % $D_1 = |g_1 \rangle \langle e|$  and $D_2 = |g_2 \rangle \langle e|$.  The interaction Hamiltonian is 
% % \begin{gather}
% % H_\text{eff} = \frac{1}{2(\Delta - i \Gamma/2)} \left(\Omega_1 D_1 e^{-i k_1 \hat{x}}  + \Omega_2 D_2 e^{-i k_2 \hat{x}}   \right)  \\
% % \times | \rangle e,n'\rangle  \langle e,n'| \left(\Omega_1 D_1^\dag e^{i k_1 \hat{x}}  + \Omega_2 D_2^\dag e^{i k_2 \hat{x}}   \right)  \nonumber \\
% % =    \frac{1}{2(\Delta - i \Gamma/2)} \left(   \Omega_1^2 |g_1 \rangle \langle g_1|      +   \Omega_1^2 |g_2 \rangle \langle g_2|    +   \right. \\
% %   \left. \Omega_1 \Omega_2 ( D_1 e^{- i k_1 x}  |n',e \rangle \langle n',e |  D_2^\dag e^{ i k_2 \hat{x} }    )  \right)
% % \end{gather}
% % First two terms are light shift.  The coupling between $g_1$ adn $g_2$ is 
% % \begin{gather}
% %     \langle g_1, n_1 | H_\text{eff} | g_2, n_2 \rangle = \\
% %     \frac{\Omega_1\Omega_2}{\Delta - i \Gamma/2}  \sum_{n'}   \langle g_1, n_1|  D_1 e^{ - i k_1 x}  | e, n' \rangle \langle e, n'| D_2 e^{ i k_2 x}  | g_2, n_2 \rangle    \\
% %     = \frac{\Omega_1\Omega_2}{\Delta - i \Gamma/2}    \langle n_1|  e^{ - i (\bm{k_1}-\bm{k_2}) \cdot \bm{r} }  | n_2 \rangle    
% % \end{gather}
% % When $k_1 = k_2$, cannot change $n$.  Anayltical expression?



% % The collapse operators are
% % \begin{gather}
% %     L_{eff, 1} = \sqrt{\Gamma} e^{\pm ikx} D_1 \left( \Omega_1 D_1^\dag e^{-i k_1 \hat{x}}  + \Omega_2 D_2^\dag e^{-i k_2 \hat{x}} \right)   \\
% %     L_{eff, 2} =   \\
% %     L_\text{eff, S}  =  \sqrt{\gamma_S} |g_1 \rangle \langle g_2 |
% % \end{gather}
% % Last one is spontaneous emission. 

% % The effective model is simply 

 

% % Raman sideband cooling also uses two coherent lasers to couple two different ground states.  In EIT cooling, those same lasers provided the optical pumping between those two states. In Raman sideband cooling, the single photn detuning is typicaly increased until scattering is much smaller than the Rabi coupling.  Then a third lasers is incorporated that provides the optical pumping from $|g_2 \rangle$ to $|g_1 \rangle$.   Selection rules are typicall used so that it pumps back to $g_1$, but then $g_1$ is dark to the optical pumping light.  Then only a the minimum number of scattering evens i sused to reset the population.  

% % The final temperature is. 
% % \Jon{work out CW and digital cases.  How large of detuning to get ground state. Could we do 1 GHz detuning?}


% % \section{Appendix}

% % \subsection{Appendix A: Adiabatic Elimination of the Excited State}
% % \label{app:adiabatic}
% % \Jon{I go back and forth about including this.}
% % equilvanet to expressing the equations of motions for ground adn excited, then integrating the excited equation and sbutituting it into the ground state.  Then making an assumption about time scale of evolution in ground state. 

% % The adiabatic elimination of the excited state involves slaving the excited state to the ground state. The excited state is solved in terms of the ground state, and then used to eliminate the excited state dependence in the evolution of the ground state, as in the formalism in Ref.~\cite{deutsch2010quantum}. A more general formalism for adiabatic elimination was developed in Ref.~\cite{reiter2012effective}, which we follow here. Adiabatic elimination is accurate when the time evolution of the wavefunction is slow compared to the excited state decay rate. Since cooling typically occurs on time scales much longer than the decay rate, this is generally an excellent approximation for limits typical of cooling: low-saturation and far-detuning. Here we provide a brief summary of the formalism and then apply it to the laser cooling Hamiltonian.

% % The total Hamiltonian is 
% % \begin{equation}
% %     H = H_e + H_g + V^+ + V^-
% % \end{equation}

% % Each term can be expressed in terms of ground and excited state projection operators $P_g$ and $P_e$ as 
% % \begin{gather}
% %    H_e = P_e H P_e, \quad H_g = P_g H P_g,  \nonumber \\
% %    V^+ = P_g H P_e, \quad V^- = P_e H P_g.
% % \end{gather}


% % The decay of the excited state is incorporated in the Wigner-Weisskopf picture by including decay terms in a non-Hermitian Hamiltonian 
% % \begin{gather}
% % H_\text{NH} = H_e - \frac{i}{2} \sum_i \hat{L}_i^\dag \hat{L}_i.
% % \end{gather}
% % $L_i$ are the collapse operators coming from spontaneous emission.
% % For the case of free-space spontaneous emission from an atom, all levels decay with the same rate $\Gamma$ and 
% % \begin{equation}
% %     H_\text{NH} = H_e - i \frac{\Gamma}{2} P_e
% % \end{equation}


% % The master equation for the time evolution of the density matrix also includes a re-feeding term that brings the population back to the ground state
% % \begin{gather}
% %     \dot{\rho} = - i (H_\text{NH} \rho - \rho H_\text{NH}^\dag ) + \sum_q L_q \rho L_q^\dag .
% % \end{gather}
% % In situations where the excited state quickly reaches an equilibrium, the excited state can be solved in terms of the grounds states and then eliminated from the time evolution equations.  The elimination results in an effective Hamiltonian and jump operator that give the dynamics within the ground state.  These effective operators can be derived by performing these operators for a given Hamiltonian, but Ref.~\cite{reiter2012effective} provides a compact general formalism which we use.  The effective operators are
% % \begin{gather}
% % H_\text{eff} = \nu a^\dag a  \nonumber \\ 
% % -  \frac{1}{2} \left[V^- \sum_{m_g} \frac{1}{(H_\text{NH} - E_{m_g})} V^+ |m_g \rangle \langle m_g |   
% % + h.c. \right]  
% % \end{gather}
% % \begin{gather}
% % L_\text{eff}^i = L_i \sum_{m_g} \frac{1}{(H_\text{NH} - E_{m_g})} V^+ | m_g \rangle \langle m_g |.
% % \end{gather}
% % Here, $|m_g \rangle$ are the eigenstates of the ground state manifold with corresponding energy $E_{m_g}$.
% % These operators can also be written in terms of the excited state eigenstates $|m_e \rangle$ with corresponding energies $\Delta_e$ by inserting a sum over all excited states,
% % \begin{gather}
% % H_\text{eff} = \nu a^\dag a \nonumber \\
% % -\frac{1}{2} \left[ \sum_{m_g,m_e} \frac{V^-|m_e \rangle \langle m_e|V^+}{( \Delta_{m_e, m_g} - i \Gamma/2 )} |m_g \rangle \langle m_g |   
% % + h.c. \right] 
% % \end{gather}
% % \begin{gather}
% % L_\text{eff}^i =  L_i \sum_{m_g, m_e} \frac{ |m_e \rangle \langle m_e| V^+}{\Delta_{m_e, m_g} - i \Gamma/2}  | m_g \rangle \langle m_g |.
% % \end{gather}
% % The laser detuning is $\Delta_{m_g,m_e} = \omega_L - (E_{m_e} - E_{m_g} ) $.  
% % The effective Hamiltonian includes light shifts, two-photon Raman coupling, and decay due to spontaneous emission. The jump operators repopulate the ground state. 



% % In the further approximation that the ground state detunings are small compared to the laser detuning, the sum over $m_g$ converts to an identity, leading to a simpler expression:
% % \begin{equation}
% %     H_\text{eff} = -\frac{1}{2} V_- \left[H_\text{NH}^{-1} + (H_\text{NH}^{-1})^\dag \right]V_+ + H_g
% % \end{equation}
% % \begin{equation}
% %     L_\text{eff}^q = L_q H_\text{NH}^{-1} V_+
% % \end{equation}

% % Now, considering the case of laser cooling of an atom, the initial Hamiltonian is:
% % \begin{gather}
% %     V_+ = - \frac{\Omega}{2} (\bm{\epsilon}(\hat{x}) \cdot \bm{D}) ,  \quad V_- = V_+^\dag\\
% %     L_{q, \bm{n}} = (\mathcal{R}_{\bm{n}}  \, \hat{\bm{e}}_q^*) \cdot \bm{D}
% % \end{gather} 
% % The non-Hermitian excited state Hamiltonian is
% % \[H_\text{NH} = \sum_{m_e} \left(\Delta_{m_e} - i \frac{\Gamma}{2} \right) |m_e \rangle \langle m_e|\]
% % where $|m_e \rangle$ are the eigenstates of the excited state with energies $E_{m_e}$.  

% % Substituting these into the effective Hamiltonian gives
% % \begin{gather}
% % H_\text{eff} = \nu a^\dag a - \\
% % \frac{\Omega^2}{8} \left[ 
% %   \sum_{m_g,m_e} \frac{ (\bm{\epsilon}
% % (\hat{x}) \cdot \bm{D}) |m_e \rangle \langle m_e | (\bm{\epsilon}^*(\hat{x}) \cdot \bm{D}^\dag)}{(\Delta_{m_g,m_e} - i \Gamma/2 )}   
% %  |m_g \rangle \langle m_g | + h.c. \right] 
% % \end{gather}
% % and the jump operator for the emission of a photon with polarization $q$ is:
% % \begin{gather}
% % L_\text{eff}^{q, \bm{n}} = - \frac{\Omega}{2} \sum_{m_g, m_e} \frac{ (\mathcal{R}_{\bm{n}} \bm{e}_q^* \cdot \bm{D})|m_e \rangle \langle m_e| (\bm{\epsilon}(\hat{x}) \cdot \bm{D}^\dag)}{ \Delta_{m_g,m_e} - i \Gamma/2} | m_g \rangle \langle m_g |
% % \end{gather}

% % In the large detuning limit, the state dependence in the denominator goes away, and the sum over the excited states in the numerator becomes the identity.  The effective operators simplify to 
% % \begin{gather}
% % H_\text{eff} = \nu a^\dag a - 
% % \frac{\Omega^2}{4} \left[ 
% %    \frac{ (\bm{\epsilon}^*(\hat{x}) \cdot \bm{D}) (\bm{\epsilon}(\hat{x}) \cdot \bm{D}^\dag)}{\Delta - i \Gamma/2 } \right] 
% % \end{gather}
% % and
% % \begin{gather}
% % L_\text{eff}^{q,\bm{n}} = - \frac{\Omega}{2} \frac{ ( \mathcal{R}_{\bm{n}} \bm{e}_q^* \cdot \bm{D}) (\bm{\epsilon}(\hat{x}) \cdot \bm{D}^\dag)  }{ \Delta - i \Gamma/2}  . 
% % \end{gather}
% % What about multiple frequencies?

% % When the detuning of the laser is large compared to the energy splittings of the ground and excited states, then we can take $\Delta_{m_g,m_e}  \approx \Delta $,  and then we can replace the sums $\sum_{m} |m \rangle \langle m | $ with the identity for both the ground and excited, leading to simpler expressions for the ground state dynamics in the large detuning limit
% % \begin{gather}
% % H_\text{eff} = -\frac{1}{2} \left[ \frac{V^-V^+}{( \Delta - i \Gamma/2 )}   
% % + h.c. \right] + \nu a^\dag a 
% % \end{gather}
% % \begin{gather}
% % L_\text{eff}^i = L_i \frac{   V^+}{\Delta - i \Gamma/2}  .
% % \end{gather}


% % \subsubsection{Unknown}
% % I'm not sure where there should go rightnow. 

% % We can now use

% % \begin{gather}
% % \gamma_{m_g \rightarrow m_g' } = 
% % \Gamma \frac{\Omega^2}{4} \left| \sum_{m_e, \bm{n}} \frac{  \langle m_g' | ( \mathcal{R}_{\bm{n}}\bm{e}^*_q \cdot \bm{D}) |m_e \rangle \langle m_e | (\bm{\epsilon}(\hat{x}) \cdot \bm{D}^\dag) | m_g \rangle }{\Delta_{m_g, m_e} - i \Gamma/2}  \right|^2
% % \end{gather}

% % The average over the spontaneous emission angles generally cancels out the cross-terms, so that the sum over rexcited states can be brought out of hte magnitude. 
% % We also define 
% % scattering rate 
% % \begin{equation}
% %     R( \Delta ) = \Gamma \frac{\Omega^2}{\Delta^2 + \Gamma^2 /4 }
% % \end{equation}

% % \begin{gather}
% % \gamma_{m_g \rightarrow m_g' } = \sum_{m_e}  R(\Delta_{m_g,m_e})  
% % \times \left|  \langle m_g' | (e^{i k x}\bm{e}^*_q \cdot \bm{D}) |m_e \rangle \langle m_e  | (\bm{\epsilon}(\hat{x}) \cdot \bm{D}^\dag) | m_g \rangle \right|^2
% % \end{gather}

% % \begin{equation}
% % \gamma_{m_g \rightarrow m_g' } = \frac{\Omega^2}{4( \Delta^2 + \Gamma^2/4)} \left| \langle m_g' | (e^{\pm i k x}\bm{e}^*_q \cdot \bm{D} )( \bm{\epsilon}(\hat{x}) \cdot \bm{D}^\dag) | m_g \rangle \right|^2
% % \end{equation}
% % where $m_g$ and $m_e$ represent the motional and spin states of the ground and excited states, respectively. 




% % The last term assumes that the emitted light can only propagate in $\pm x$ direction. Full expression is an integral over all solid angles
% % \begin{equation}
% %  \Gamma \int d \Omega_n N(\bm{n}) e^{i |k|  \bm{n} \cdot \hat{\bm{x}}} D_q \rho D_q^\dag e^{-i |k| \bm{n} \cdot \hat{\bm{x}}}
% % \end{equation}

% % In the master equation, the density matrix is repopulated with the collapse operators $\sqrt{\gamma_j} \hat{C}_j $  through the  terms  $\frac{1}{2} \sum_i \gamma_j C_i  \rho C_i^\dag$.  
% %For the case of spontaneous emisison in three dimensions,  $\sqrt{\gamma_j} c_j \rightarrow \sqrt{\gamma N_\bm{n} } D  e^{i \bm{k}_\bm{n} \cdot \bm{r} }$.   
% %The sum becomes an integral over all solid angles $\int d \Omega_{\bm{n}} N_\bm{n} e^{i k \hat{\bm{n}} \cdot \bm{x} } D \rho  D^\dag   e^{-i k \hat{\bm{n}} \cdot \bm{x} } $, where $\hat{\bm{n}}$ is the unit propagation direction and $N_\bm{n}$ is the the angular distribution.  
% % To simplify the formalism in one dimensions, we will assume the ligh is only emitted in $\pm \hat{z} $, in which case  $\hat{C}_\pm =  \hat{D} e^{\pm i k \hat{z}} $. 


% % In Raman-sideband cooling, the lasers are far detuned from the excited states, so the scattering is much smaller than the Raman coupling.  Typically, the two ground states $|g_1 \rangle $ and $|g_2 \rangle$ are also far detuned from each other, for example, within different hyperfine ground states, such that the two lasers only address one transition.  As shown in Fig.~\ref{}, two beams with different frequencies  $\bm{E}_1 e^{i \bm{k}_1 \cdot \bm{r} } $ and $\bm{E}_2 e^{i \bm{k}_2 \cdot \bm{r} } $ address the two ground states with the corresponding detunings $\Delta_1$ and $\Delta_2$ from the excited state.  Two-photon detuning $\delta = \Delta_1- \Delta_2 $ is set to $-\nu$ to drive $|g_1, n \rangle \rightarrow |g_2, n-1 \rangle$.  Because spontaneous emission is suppressed, optical pumping back to $|g_1, n \rangle$ is achieved at another frequency close to resonance with an excited state.


% %which can even be made dark for the $|g_1, n \rangle$ state due to polarization and angular momentum selection rules. 
% %RSB has been covered in many references, but we review the formalism here to aid in understanding the later schemes. 
% % In the large detuning limit, the excited states can be eliminated, which leads to effective two-level system Raman coupling between the two ground states $\Omega_R$.  We include multiple electronic ground states, for example, different hyperfine states and different harmonic oscillator states $|e_k, n'' \rangle $ with trapping frequency $\nu_e$, which can differ from the ground state trapping frequency. However, we assume that the two ground states share the same potential. %, although this may not hold in the presence of vector and tensor shifts.
% % The total Raman coupling between states $|g_1, n \rangle $ and $|g_2, n' \rangle $ has to be summed over all the excited states $|e_k, n'' \rangle $ with the corresponding detunings $\Delta_k + n'' \nu_e$, where $\Delta_k$ is the detuning from the $e_k$ state,
% % %
% % \begin{equation}
% % \tiny
% %     \Omega_{n, n'}  = \sum_{n'', k}  \frac{ \langle g_1, n| (\bm{E}_1\cdot \bm{D}_2) e^{i \bm{k}_1\cdot \bm{r} } | e_k , n'' \rangle  \langle e_k, n''| (\bm{E}_2^*\cdot \bm{D}_1 ) e^{-i \bm{k}_2\cdot \bm{r} } | g_2 , n' \rangle }{\Delta_k +  \nu_e n''  } 
% % \end{equation}
% % %


% % Because the motional states do not affect the electronic transitions, we can separate the electronic and motional components and define the electronic Rabi frequencies 

% % When $\Delta_k \gg \nu_e$, we can ignore $\nu_e$ in the denominator and separate the sums as shown below
% % %
% % \begin{gather}
% %    \Omega_{n, n'} \approx \sum_{e_k}  \Omega_1 \Omega_2 \frac{ \langle g_1 |  (\bm{\epsilon}_1\cdot \bm{D}) | e_k \rangle \langle e_k |  (\bm{\epsilon}^*_2\cdot \bm{D}) | g_2 \rangle      }{ \Delta_k} \,\   \\
% %    \times \,\, \sum_{n''}  \langle n | e^{i(\bm{k}_1)\cdot \bm{r}}  | n'' \rangle \langle n'' | e^{-i(\bm{k}_2)\cdot \bm{r}}  | n' \rangle
% % \end{gather}    %check this.  wave-vector sign?
% % %
% % Then we can replace  $\sum_{n''} | n'' \rangle \langle n'' | $ with the identity and define the electronic Raman coupling $\Omega_R$ as the first electronic sum to get
% % %
% % \begin{equation}   \label{eq:Omegann}
% %    \Omega_{n, n'} = \,\ \Omega_R  \, \times  \, \langle n | e^{i(\bm{k}_1 -\bm{k}_2)\cdot \bm{r}} | n' \rangle
% % \end{equation}
% % %
% % This is the Raman Rabi coupling between $|g_1, n \rangle $ and $|g_2, n' \rangle$. It has the property that $\Omega_{n,n'} = \Omega_{n',n}$. The coupling is similar to the single-photon transition, with $\bm{k}_1 - \bm{k}_2$ playing the role of the wavevector. 

% % If the single photon detuning $\Delta_k$ is similar for all excited states, then we can also replace $\sum_{e_k} |e_k \rangle \langle e_k |$ with the identity to give 
% % \begin{equation} \label{eq:OmegaR}
% %     \Omega_R =  \frac{\langle g_1 |(\bm{E}_1\cdot \bm{d})  (\bm{E}_2^*\cdot \bm{d}^*)  |g_2 \rangle}{\Delta}
% % \end{equation} % Check this.

% % After the Raman coupling between $|g_1, n \rangle $ and $|g_2, n-1 \rangle$, the ground state must be optically pumped back to $g_1$ to repeat the cycle, which is achieved by a near-resonant optical pumping beam with a rate $\gamma_p$.  For a two-photon transition between two stable ground states, the effective linewidth of the transition is determined by this pumping rate, and we can define a scattering rate between $|g_1, n \rangle $ and $|g_1, n' \rangle$ as 
% % %
% % % \begin{equation}  \label{eq:Ann}
% % %     A_{n,n'} = \gamma_p \frac{ (\Omega_{n,n'}/\gamma_p)^2}{ 1 + 2 (\Omega_{n,n'}/\gamma_p)^2 + 4 \delta ^2/\gamma_p^2  }
% % % \end{equation}
% % %
% % where $\delta$ the two-photon Raman detuning. 
% % For pulsed Raman sideband cooling, optical pumping is performed in a separate stage and $\pi/2$ pulse, where $\Omega_R$ sets the linewidth. 
% % % \begin{equation}
% % %   \frac{\Omega}{1 + \Delta}  \sin^2( \sqrt{\Delta^2 + \Omega^2}  t)
% % % \end{equation}
% % %
% % %Just as in the Doppler case, we can derive the population rate equations
% % % \begin{gather}
% % %     \frac{d P(n)}{dt} = - P(n) \left[ A_{n,n-1} + A_{n,n+1} +\eta^2 (2n+1) (A_{nn} + \gamma_s ) \right]  \nonumber \\
% % %     + P(n+1) \left[ A_{n+1,n} + \eta^2 (n+1)(A_{n+1,n+1} + \gamma_s)  \right]  \nonumber \\
% % %     +P(n-1) \left[   A_{n-1,n} + \eta^2 n (A_{n-1,n-1} + \gamma_s)   \right]
% % % \end{gather}


% % % We can then just as before calculate a rate equation for $\langle n \rangle $
% % % \begin{equation}
% % %     \frac{d \langle n \rangle}{dt} = \langle A_{n,n+1} \rangle - \langle A_{n,n-1} \rangle  + \eta^2  ( \langle A_{n,n} \rangle + \gamma_s) 
% % % \end{equation}
% % % The ratio of the ground state to the first state has the simple form 
% % % \begin{equation}  \label{eq:P0P1}
% % %     \frac{P(0)}{P(1)} = \frac{A_{1,0} + \eta^2(A_{1,1} + \gamma_s ) }{  A_{0,1} + \eta^2(A_{0,0} + \gamma_s)}
% % % \end{equation}
% % % This cooling equation helps us derive a lower-bound temperature limit for each cooling scheme.    The ratio $A_{1,0}/A_{0,1}$ simply indicates how well you can resolve the $n \rightarrow n-1$ transition over $n \rightarrow n+1$.   The terms on the rate in the numerator and denominator are simply due to scattering from either driving the $|g_1, n \rangle \rightarrow |g_2, n \rangle $ transition or any other excess scattering, such as off-resonant scattering from the $|g_2 \rangle $ if detuning is not sufficiently large. 




%  %\frac{n \, \Omega^2}{(\gamma_{+} + \gamma_{-} ) }$.   
% % This doesn't scale with detuning, meaning that at large detuning the scattering decreases, and eventually this will dominate.  In this limit, then the raman coupling between states will dominate and they will be in equilibrium. 
% %
% % \Jon{will take this equation out}
% % \begin{align*}
% % \dot{P}_-(n) = - (\gamma_{+} + n \eta^2  A) P_-(n) + \\
% %     \gamma_{-} P_+(n) +n  \eta^2 A \, P_-(n-1)   \\
% %     \\
% % \dot{P}_+(n) = \frac{n \, \Omega^2}{(\gamma_{+} + \gamma_{-} ) } \left[ P_-(n-     1) - P_+(n) \right] \\
% %     - (\gamma_{-} +n \, \eta^2 A )P_+(n) + \gamma_{+} P_-(n) + \eta^2 n A P_+(n+1) \\
% %     \\
% % \dot{P}_-(n-1) = \frac{- n \, \Omega^2}{(\gamma_{+} + \gamma_{-} ) } \left[ P_-    (n-1) - P_+(n) \right] \\
% %     - (\gamma_{+} + n \, \eta^2 A )P_-(n-1) + \gamma_{-} P_+(n-1) + \eta^2 n A P_-(n)  \\
% %     \\
% % \dot{P}_+(n-1) = - (\gamma_{-} + \eta^2 n A) P_+(n) + \\
% %     \gamma_{+} P_-(n) +n  \eta^2 A \, P_+(n)  
% % \end{align*}
% % here
% % $\Omega = \eta V_0$,   $\gamma_{-} = \Gamma  \frac{\Omega^2/4}{\Delta^2 + (\Gamma/2)^2}$.
% % $\gamma_s = \Gamma \frac{\Omega^2/4}{\Delta^2) + (\Gamma/2)^2}$
% %
% % In steady-state we can look at just two levels and invoke that there should be no flow between these two states. We can do this because in LD regime only neibroing $n$ are coupled
% % \begin{align*}
% %  (\gamma_{+} + n \eta^2  A) P_-(n) =  
% %     \gamma_{-} P_+(n) +n  \eta^2 A \, P_-(n-1)   \\
% %     \\
% %  \left[ \frac{n \, \Omega^2}{(\gamma_{+} + \gamma_{-} ) } + (\gamma_{-} +n \, \eta^2 A ) \right] \,\, P_+(n) =  \\
% %  \frac{n \, \Omega^2}{(\gamma_{+} + \gamma_{-} ) } \left[ P_-(n-     1)   \right] + \gamma_{+} P_-(n) + \eta^2 n A P_+(n+1) \\
% %     \\
% %  \left[ \frac{- n \, \Omega^2}{(\gamma_{+} + \gamma_{-} )} + (\gamma_{+} + n \, \eta^2 A )  \right] \,\, P_-(n-1) = \\
% %  -\frac{ n \, \Omega^2}{(\gamma_{+} + \gamma_{-} ) } \, P_+(n)  +
% %     \gamma_{-} P_+(n-1) + \eta^2 n A P_-(n)  \\
% %     \\
% %  (\gamma_{-} + \eta^2 n A) P_+(n) = \gamma_{+} P_-(n) +n  \eta^2 A \, P_+(n)   
% % \end{align*}
% % In the limit of $\Omega \rightarrow \infty$, where the transfer from $\Omega$ is much larger than the scattering rate,  then the middle two equations are require $P_+(n) = P_-(n-1)$.  We are then just left with the top and bottom equation.
% % In the limit where the $\frac{\Omega^2}{\gamma_{01} + \gamma_{10} } \rightarrow \infty$, which is achieved by going to large detuning bacuse scattering scales as $1/\Delta^2$ and the coherence coupling $\Omega$ scales as $1/\Delta$.  In this limit $P_-(n) = P_+(n-1)$, because at large enough detuning, this transfer rate will be largest, because also other scattering scales as $1/\Delta^2$.


% % All scattering is on order $\gamma \sim \Gamma \frac{\Omega^2}{4 \Delta^2}$.  In large detuning limit, detuning cancels out.  In the limit that of $F=1$ to $F=1$ cooling where state is really dark, then $\gamma_{-} = 0$, and we get 
% % \begin{equation}
% %     \frac{P(1)}{P(0)} = \frac{1}{1 + \gamma_{+}/ \eta^2 \gamma_r}   \approx  \frac{\eta^2}{1 + \eta^2}
% % \end{equation}
% % Even in limit of $\eta = 0.1$, leads to signficant ground state population. 


% % However in limit of PG cooling where weak assymetry in optical pumping, not dark, then limit is 
% % \begin{equation}
% %     P(1)/P(0) \approx  \gamma_{-}/ \gamma_{+}
% % \end{equation}





% % \Jon{below is temporary and for multipel fields}
% % \begin{equation}
% % \hat{H}_{\text{eff}} = -\frac{1}{2} \Bigg[ \mathbf{\hat{V}}_{-} \sum_{f,l} \left( \hat{H}_{NH}^{(f,l)} \right)^{-1}  \mathbf{\hat{V}}_{+}^{(f,l)}(t) + \text{H.c.} \Bigg] + \hat{H}_g,
% % \end{equation}

% % \begin{equation}
% % \mathcal{L}_k^{\text{eff}} = \mathcal{L}_k \sum_{f,l} \left( \hat{H}_{NH}^{(f,l)} \right)^{-1}  \mathbf{\hat{V}}_{+}^{(f,l)}(t),
% % \end{equation}

% % \begin{equation}
% % \left( \hat{H}_{NH}^{(f,l)} \right)^{-1} = \left( \hat{H}_{NH} - E_l - \omega_f \right)^{-1}.
% % \end{equation}



% \subsection{Appendix: Cooling rate equations}
% \label{app:rate}
% \Jon{get rid of this}
% Appendix~\ref{} presented an effective Hamiltonian and jump operator for ground state dynamics. To approximate cooling rates and temperatures, it is useful to derive rate equations between the ground state spin and motional states. We start with a master equation that describes the ground state in the interaction picture  dynamics \textcolor{red}{Maybe use tilde for interaction picture?}
% \begin{equation}
% \dot{\rho} =  \sum_i \left[ L_i \rho L_i^\dag - \frac{1}{2} \{ L_i^{\dag} L_i , \rho \} \right]
% \end{equation}
% % \begin{equation}
% % \dot{\rho} = - i (H \rho - \rho H ) +    \sum_i \left( L_i \rho L_i^\dag - \frac{1}{2} \{ L_i^{\dag} L_i , \rho \} \right)
% % \end{equation}
% The Hamiltonian here is Hermitian, and the non-Hermitian parts have been put in the anti-commutator of the Lindbaldian.   In the interaction picture, the time evolution of the Hamiltonian is put within the density matrix and operators  $ U \rho U^\dag$ with unitary $U = e^{-i H t}$.  

% We can determine the population by multiplying by $\langle n |$ on the left and $| n \rangle$ on the right, defining $P(n) = \rho_{nn}$. We then eliminate all the coherences $\langle n | \rho | m \rangle$, resulting in:
% \begin{gather}
% \frac{dP(m)}{dt}
% = - P(m) \sum_{n,i}|\langle n | L_i | m \rangle|^2 \
% + \sum_{n,i} P(n) |\langle m | L_i | n \rangle|^2.
% \end{gather}
% We define the transfer rate between ground states $n$ and $m$ as:
% \begin{equation}
% \gamma_{n \rightarrow m} = |\langle m | L_i | n \rangle|^2 .
% \end{equation}
% It is important to note that in this definition, whether $L_q$ is in the interaction picture or not is irrelevant, as any extra phase cancels out upon taking the magnitude. The resulting rate equation is then:
% \begin{equation}
% \frac{dP(n)}{dt} = - P(n) \sum_{m} \gamma_{n \rightarrow m} + \sum_{m} \gamma_{m \rightarrow n} P(m)
% \end{equation}
% However, caution is advised with this approximation, as it disregards coherences between all levels. For instance, it is not applicable in scenarios such as a two-photon Raman transfer between states or if working outside a diagonal basis. The approximation holds when spontaneous emission primarily drives population transfer between states.
% The rate equation is can be represented as a matrix equation and solve for the steady state solution  $\frac{dP(n)}{dt} = 0$.



% \subsection{Derivation of J master equation}
% Before diving into the derivation, first we work out the dipole moment operator and electric field operator in the preferred basis.  The atom-dipole notation follows the conventions of Ref.~\cite{steck}. 
% The dipole operator is expressed in spherical vector form as
% \begin{equation}
% \mathbf{d} = \sum_q d_q \hat{\mathbf{e}}_q^*,
% \end{equation}
% with components $d_{\pm1} = \mp \frac{1}{\sqrt{2}} (d_x \pm i d_y)$ and $d_0 = d_z$. The unit spherical vectors are similarly defined as $\hat{\mathbf{e}}_{\pm1} = \mp \frac{1}{\sqrt{2}} (\hat{\mathbf{e}}_x \pm i \hat{\mathbf{e}}_y)$ and $\hat{\mathbf{e}}_0 = \hat{\mathbf{e}}_z$. Spherical vectors possess properties such as $(d_q)^* = (-1)^q d_{-q}$ and dot product $\mathbf{A} \cdot \mathbf{B} = \sum_q (-1)^q A_q B_{-q} = \sum_q A_q B_q^*$, with orthogonality $\hat{e}_q \cdot \hat{e}_{q'}^* = \delta_{qq'}$.

% The identity operator in the atom basis is a sum of all ground and D1 excited states:
% \begin{equation}
% \hat{\mathcal{I}} = \sum_{m_g} |J_g m_g \rangle \langle J_g m_g | + \sum_{m_e} |J_e m_e \rangle \langle J_e m_e |.
% \end{equation}
% Multiplying the dipole operator on both sides by the identity $\hat{\mathcal{I}} d_q \hat{\mathcal{I}}$ and using the Wigner-Eckert theorem and angular momentum identities yields an expression for the dipole momentum operator in terms of a collective lowering operator $\Sigma_q$~\cite{steck}:
% \begin{equation}
% d_q = \langle J_g || d || J_e \rangle \left(\Sigma_q + (-1)^q \Sigma_{-q}^\dag \right) = d_q^{(+)} + d_q^{(-)}.
% \end{equation}


% \begin{equation}
% \Sigma_{q} = \sum_{m_g m_e} \langle J_g m_g|J_e m_e ; 1 q \rangle \,\,
%  |J_g m_g \rangle \langle J_e m_e|.
% \end{equation}
% %
% The electric field operator written in complex form with a rotating $(+)$ and counter rotating  $(-)$ terms is 
% \begin{equation}
% \mathbf{E}(\mathbf{r} , t) = \mathbf{E}^{(+)}(\mathbf{r} , t) + \mathbf{E}^{(-)}(\mathbf{r} , t) =  \left(  \boldsymbol{\mathcal{E}}^{(+)}(\mathbf{r})  e^{- i \omega t}  + \text{c.c.} \right)   
% \end{equation}
% The complex spatial field is expressed in terms of a sum of plane waves
% \begin{equation}
%   \boldsymbol{\mathcal{E}}^{(+)}(\mathbf{r}) = \sum_j  \boldsymbol{\epsilon}_{j} \frac{E_{j}}{2} e^{i \mathbf{k}_{j} \cdot \mathbf{r}}  
% \end{equation}
% The index $j$ denotes the beam index for one of the frequencies, $\mathbf{k}_{j}$ is the wave-vector and beam $j$,  $\boldsymbol{\epsilon}_{j}$ is the polarization vector,  and $E_{j}$ is the complex electric field amplitude.  The intensity is related to the amplitude by $I = \frac{c \epsilon_0}{2} |E|^2 $.

% The Hamiltonian for the interaction between the atom and the electric field of the laser in the dipole approximation and rotating wave approximation (but not in the rotating frame) is
% \begin{align}
%     H_{\text{AF}} &= -\mathbf{d}^{(+)} \cdot \mathbf{E}^{(-)} - \mathbf{d}^{(-)} \cdot \mathbf{E}^{(+)} \nonumber \\
%     &= -\sum_q (-1)^q \left( d_q^{(+)} E_{-q}^{(-)} + d_q^{(-)} E_{-q}^{(+)}  \right)  
% \end{align}
% We define the position-dependent but time-independent Rabi frequencies
% \begin{equation}
%     \Omega_{q,i}(\mathbf{r}) = -2 \langle J_g || \mathbf{d} || J_e \rangle  \frac{1}{\hbar}  \mathcal{E}^{(+)}_{q,i}(\mathbf{r})
% \end{equation}
% The atom-field interaction is then defined in terms of a sum over the two laser frequencies and all three polarizations 
% \begin{equation}
%     H_{AF} = \frac{1}{2} \sum_{q} \left( \Omega_{q}(\mathbf{r}) \Sigma_q^{(+)} e^{-i\omega t} + h.c. \right)
% \end{equation}
% % labels for the F=3/2 and F=1/2 ground states.  

% by applying a unitary transformation
% \begin{equation}
%    U =  e^{- i \omega t   \sum_{m_g} |J_g,  m_g \rangle \langle J_g,  m_g |  }     
% \end{equation}
% The new Hamiltonian transforms to $ H \rightarrow   U H U^\dag + i \hbar (\frac{\delta}{\delta t} U) U^\dag$ and the operators transform to  $ \sigma  \rightarrow U \sigma U^\dag$. 
% From now on, all operators will be assumed to be in the rotating frame defined by this unitary operator.


% \subsection{Master equation in J picture}
% (incorporate this into previous section)

% In this rotating frame, the non-interacting Hamiltonian is ( excited state as zero energy) 
% \begin{equation}
%     \begin{split}  
%       H_0 &=  \sum_{m_g}  \hbar  \delta  \, |J_g, m_g \rangle \langle J_g, m_g| 
%     \end{split}
% \end{equation}

% The atom-field interaction has two terms.
% \begin{equation}
%     H_{\text{AF}} = \frac{\hbar}{2} \sum_q \left(  \Omega_{q} (\mathbf{r}) \Sigma^\dag_{q}   + h.c.   \right)
% \end{equation}

% Lastly, the interaction with motional states is incorporated by first adding a harmonic oscillator Hamiltonian. 
% \begin{equation}
% H_\text{HO} =  \hbar \omega (a^\dag a  + 1/2 )
% \end{equation}
% where $\omega$ is the trapping frequency. Second, we promote the positions in $\Omega_{q,i}(\mathbf{r})$ to operators.
% In our 1D simulation, we assume that the incoming light is propagating in the $z$ direction as $E_0 e^{ikz}$ with real amplitude $E_0$. We also assume there is a retro-reflected beam with the same magnitude $E_0 e^{i \phi }e^{ikz}$ but with a phase determined by the mirror position. We also assume that the polarization is in the $x$-$y$ plane. We define recoil operators 
% \begin{equation}
%     \hat{\mathcal{R}} = e^{i k \hat{z}}, \quad  \hat{\mathcal{R}}^\dag = e^{-i k \hat{z}}
% \end{equation}
% which are momentum displacement operators corresponding to a recoil from photon absorption or emission. 
% We do not assume the Lamb-Dicke (LD) regime in our simulations, but we find it useful to expand the recoil operator in the LD regime to see what the dominant terms correspond to. The LD regime here would correspond to the expansion
% \begin{equation}
%     \hat{\mathcal{R}} \approx  1 + i k \hat{z} = 1 + i \eta (\hat{a} + \hat{a}^\dag)
% \end{equation}
% where $\eta = k z_0 $ and $z_0 = \sqrt{\hbar/2m\omega}$.  The first term corresponds to no motional state change, and the second term to either the motional state gaining or loosing one quanta.

% In terms of the recoil operators, the complex electric field can be expressed as 
% \begin{equation}
%    \Omega_{q}( \hat{z}) = \Omega \left[ \epsilon_{q, \rightarrow} \hat{\mathcal{R}} + e^{i \phi} \epsilon_{q, \leftarrow} \hat{\mathcal{R}}^\dag \right]
% \end{equation}
% with scalar Rabi frequency 
% \begin{equation}
%     \Omega = -\frac{2}{\hbar} \langle J_g || \mathbf{d} || J_e \rangle \frac{E_{0}}{2}
%  \end{equation}
% %The arrow denotes whether the beam is going to the right (positive $z$) or left (negative $z$).
% The arrows denote the direction of the beam. 

% The atom-field interaction that couples the ground and excited state and motional states for a pair of counter-propagating beams is 
% \begin{equation}
%     H_{AF} = \sum_{q} \frac{\hbar \Omega}{2}  \left[ (    \epsilon_{q, \rightarrow} \hat{\mathcal{R}} + e^{i \phi} \epsilon_{q, \leftarrow} \hat{\mathcal{R}}^\dag     ) \Sigma_q^\dag + h.c.   \right]
% \end{equation}
% These equations can be used to simulate any combination of forward and backward polarizations.

% For the master equation, we use the six collapse operators corresponding to an emission of a photon with polarization $q$ in either the forward or backward direction:
% \begin{equation}
%  \hat{C}_q =  \sqrt{\Gamma} \, {\Sigma}_q,    \hat{\mathcal{R}},  \quad   \sqrt{\Gamma}  \, \Sigma_q   \hat{\mathcal{R}}^\dag
% \end{equation}
% Lindbladian
% \begin{equation}
%     \mathcal{L}_{\hat{C}} [\rho] = -\Gamma/2 \sum_j  \left(  \hat{C}^\dag \hat{C} \rho + \hat{C}^\dag \hat{C} \rho  -  2 \hat{C}^\dag \rho \hat{C} \right)  
% \end{equation}





% \section{Cooling in alkali atoms}
% \Jon{This will be in SM. }
% \subsubsection{Master Equation Derivation}
% %
% Before diving into the derivation, first we work out the dipole moment operator and electric field operator in the preferred basis.  The atom-dipole notation follows the conventions of Ref.~\cite{steck}. 
% The dipole operator is expressed in spherical vector form as
% \begin{equation}
% \bm{d} = \sum_q d_q \hat{\bm{e}}_q^*,
% \end{equation}
% with components $d_{\pm1} = \mp \frac{1}{\sqrt{2}} (d_x \pm i d_y)$ and $d_0 = d_z$. The unit spherical vectors are similarly defined as $\hat{\bm{e}}_{\pm1} = \mp \frac{1}{\sqrt{2}} (\hat{\bm{e}}_x \pm i \hat{\bm{e}}_y)$ and $\hat{\bm{e}}_0 = \hat{\bm{e}}_z$. Spherical vectors possess properties such as $(d_q)^* = (-1)^q d_{-q}$ and dot product $\bm{A} \cdot \bm{B} = \sum_q (-1)^q A_q B_{-q} = \sum_q A_q B_q^*$, with orthogonality $\hat{e}_q \cdot \hat{e}_{q'}^* = \delta_{qq'}$.



% The identity operator in the atom basis is a sum of all ground and D1 excited states:
% \begin{equation}
% \hat{\mathcal{I}} = \sum_{F_g m_g} |F_g m_g \rangle \langle F_g m_g | + \sum_{F_e m_e} |F_e m_e \rangle \langle F_e m_e |.
% \end{equation}
% Multiplying the dipole operator on both sides by the identity $\hat{\mathcal{I}} d_q \hat{\mathcal{I}}$ and using the Wigner-Eckert theorem and angular momentum identities yields an expression for the dipole momentum operator in terms of a collective lowering operator $\Sigma_q$~\cite{steck}:
% % \begin{equation}
% % d_q = \langle J_g || d || J_e \rangle \left(\Sigma_q + (-1)^q \Sigma_{-q}^\dag \right) = d_q^{(+)} + d_q^{(-)}.
% % \end{equation}
% We further separate the collective lowering operator into a lowering operator for both ground states:
% % \begin{equation}
% % \Sigma_q = \sum_{F_g} \Sigma_{q, F_g}, 
% % \end{equation}
% with lowering operator to a single hyperfine ground state as:
% %
% % \begin{flalign}
% % &\Sigma_{q, F_g} = \sum_{m_g F_e m_e} (-1)^{F_e + J_g + I + 1} \times & \nonumber \\
% % &\quad \sqrt{(2F_e+1)(2 J_g + 1)} \langle F_g m_g|F_e m_e ; 1 q \rangle & \\
% % &\begin{Bmatrix} J_e & J_g & 1 \\ F_g & F_e & I \end{Bmatrix} |F_g m_g \rangle \langle F_e m_e|. &
% % \end{flalign}




% %
% This lowering operator lowers all excited states to the $F_g$ ground state while changing $m$ by $q$.

% %\subsubsection{Electric field operator}
% The electric field operator written in complex form with a rotating $(+)$ and counter rotating  $(-)$ terms is 
% \begin{equation}
% \bm{E}(\bm{r} , t) = \bm{E}^{(+)}(\bm{r} , t) + \bm{E}^{(-)}(\bm{r} , t) =  \sum_i  \left(  \boldsymbol{\mathcal{E}}^{(+)}_i(\bm{r})  e^{- i \omega_i t}  + \text{c.c.} \right)   
% \end{equation}
% Here $i$ denotes the frequency of the laser that addresses either the  $F=3/2$ or $F=1/2$ transition.  These frequencies are typically detuned relative to each by the ground state hyperfine splitting in order to make a $\Lambda$ system. 
% The complex spatial field for a particular frequency $i$ is expressed in terms of a sum of plane waves
% \begin{equation}
%   \boldsymbol{\mathcal{E}}^{(+)}_i(\bm{r}) = \sum_j  \boldsymbol{\epsilon}_{ij} \frac{E_{ij}}{2} e^{i \bm{k}_{ij} \cdot \bm{r}}  
% \end{equation}
% The index $j$ denotes the beam index for one of the frequencies, $\bm{k}_{ij}$ is the wave-vector for frequency $i$ and beam $j$,  $\boldsymbol{\epsilon}_{ij}$ is the polarization vector,  and $E_{ij}$ is the complex electric field amplitude.  The intensity is related to the amplitude by $I = \frac{c \epsilon_0}{2} |E|^2 $.

% %\subsubsection{Hamiltonian}


% The Hamiltonian for the interaction between the atom and the electric field of the laser in the dipole approximation and rotating wave approximation (but not in the rotating frame) is
% \begin{align}
%     H_{\text{AF}} &= -\bm{d}^{(+)} \cdot \bm{E}^{(-)} - \bm{d}^{(-)} \cdot \bm{E}^{(+)} \nonumber \\
%     &= -\sum_q (-1)^q \left( d_q^{(+)} E_{-q}^{(-)} + d_q^{(-)} E_{-q}^{(+)}  \right)  
% \end{align}
% We define the position-dependent but time-independent Rabi frequencies
% \begin{equation}
%     \Omega_{q,i}(\bm{r}) = -2 \langle J_g || \bm{d} || J_e \rangle  \frac{1}{\hbar}  \mathcal{E}^{(+)}_{q,i}(\bm{r})
% \end{equation}
% The atom-field interaction is then defined in terms of a sum over the two laser frequencies and all three polarizations 
% \begin{equation}
%     H_{AF} = \frac{1}{2} \sum_{q,i} \left( \Omega_{q,i}(\bm{r}) \Sigma_q^{(+)} e^{-i\omega_i t} + h.c. \right)
% \end{equation}
% % labels for the F=3/2 and F=1/2 ground states.  


% We now go to the rotating frame of the lasers to get rid of the time-dependence.  Because the cooling light is mostly addressing the $F=3/2$ state and the repumper is mostly addressing the $F=1/2$ state, we put the two hyperfine ground states in the rotating frame of their respective laser by applying a unitary transformation
% \begin{equation}
%    U =  e^{- i \omega_{3/2} t   \sum_{m_g} |3/2,  m_g \rangle \langle 3/2,  m_g |  }  e^{- i \omega_{1/2} t   \sum_{m_g} |1/2,  m_g \rangle \langle 1/2,  m_g  |  }   
% \end{equation}
% The new Hamiltonian transforms to $ H \rightarrow   U H U^\dag + i \hbar (\frac{\delta}{\delta t} U) U^\dag$ and the operators transform to  $ \sigma  \rightarrow U \sigma U^\dag$. 
% From now on, all operators will be assumed to be in the rotating frame defined by this unitary operator.

% In this rotating frame, the non-interacting Hamiltonian is (defining $F'=3/2$ excited state as zero energy) 
% \begin{equation}
%     \begin{split}  
%       H_0 &=  \sum_{m_g} \bigg\{ \delta_{1/2} |1/2, m_g \rangle \langle 1/2, m_g|  + \delta_{3/2} |3/2, m_g \rangle \langle 3/2, m_g|\bigg\} \\
%       &+ \sum_{m_e} \bigg\{ - \Delta'_{\text{HF}} | 1/2, m_e\rangle \langle  1/2, m_e |  + 0 \times |3/2, m_e \rangle \langle 3/2, me| \bigg\}
%     \end{split}
% \end{equation}
% As defined in the level diagram, $\Delta'_{HF}$ is the D1 excited state hyperfine splitting and is positive(negative) for GM(PG) cooling. 


% The atom-field interaction has two terms.  One is time-independent, where the cooling light only addresses the $F=3/2$ state and repumper light only addresses the $F=1/2$ state:
% % \begin{equation}
% %     H_{\text{AF}} = \frac{1}{2} \sum_q \left[  \Omega_{q, 3/2} (\bm{r}) \Sig^\dag_{q,3/2}  + \Omega_{q, 1/2} (\bm{r}) \Sig^\dag_{q,1/2}  + h.c.   \right] 
% % \end{equation}
% The other atom field interaction is the cross-coupling terms consisting of the $F=3/2$ laser addressing the $F=1/2$ transition and $F=1/2$ laser addressing the $F=3/2$ transition.  These terms still have time-dependence in the rotating frame: 
% % \begin{equation}
% %     \begin{split}
% %     H_{\text{AF}}^\text{cross} = \sum_q \Big[  &\Omega_{q, 1/2} (\bm{r})  e^{i (\omega_{3/2} - \omega_{1/2} )t} \Sig^\dag_{q,3/2} \\
% %     &+ \Omega_{q, 1/2} (\bm{r})  e^{i (\omega_{1/2} - \omega_{3/2} )t} \Sig^\dag_{q,1/2}   + h.c. \Big]   
% %     \end{split}
% % \end{equation}

% This cross-coupling will be treated later as a perturbation, which is a good approximation when $\delta \ll \Delta_{HF}$.  Since the ground state hyperfine splitting is several times larger than the detunings, they are off-resonant. 
% %\subsubsection{Harmonic states}

% % Lastly, the interaction with motional states is incorporated by first adding a harmonic oscillator Hamiltonian. 
% % \begin{equation}
% % H_\text{HO} =  \hbar \omega (a^\dag a  + 1/2 )
% % \end{equation}
% % where $\omega$ is the trapping frequency. Second, we promote the positions in $\Omega_{q,i}(\bm{r})$ to operators.
% % In our 1D simulation, we assume that the incoming light is propagating in the $z$ direction as $E_0 e^{ikz}$ with real amplitude $E_0$. We also assume there is a retro-reflected beam with the same magnitude $E_0 e^{i \phi }e^{ikz}$ but with a phase determined by the mirror position. We also assume that the polarization is in the $x$-$y$ plane. 

% In terms of the recoil operators, the complex electric field can be expressed as 
% \begin{equation}
%    \Omega_{q,i}( \hat{z}) = \Omega_i \left[ \epsilon_{q, \rightarrow} \hat{\mathcal{R}} + e^{i \phi_i} \epsilon_{q, \leftarrow} \hat{\mathcal{R}}^\dag \right]
% \end{equation}
% with scalar Rabi frequency 
% \begin{equation}
%     \Omega_i = -\frac{2}{\hbar} \langle J_g || \bm{d} || J_e \rangle \frac{E_{0,i}}{2}
%  \end{equation}
% %The arrow denotes whether the beam is going to the right (positive $z$) or left (negative $z$).
% The arrows denote the direction of the beam. 

% The atom-field interaction that couples the ground and excited state and motional states for a pair of counter-propagating beams is 
% \begin{equation}
%     H_{AF} = \sum_{q,i} \frac{\Omega_i}{2}  \left[ (    \epsilon_{q, \rightarrow} \hat{\mathcal{R}} + e^{i \phi_i} \epsilon_{q, \leftarrow} \hat{\mathcal{R}}^\dag     ) \Sigma_q^\dag + h.c.   \right]
% \end{equation}
% These equations can be used to simulate any combination of forward and backward polarizations.

% % For the master equation, we use the six collapse operators corresponding to an emission of a photon with polarization $q$ in either the forward or backward direction:
% % \begin{equation}
% %  \hat{C}_q =  \sqrt{\Gamma} \, {\Sig}_q,    \hat{\mathcal{R}},  \quad   \sqrt{\Gamma}  \, \Sigma_q   \hat{\mathcal{R}}^\dag
% % \end{equation}

% Besides the cross-coupling terms which are described later, this concludes the form of the master equation used in the simulation.  The main approximations are 1) 1D motional states  2) cross-coupling scattering and shifts are small 3) photons can only be emitted in the forward and backward direction, and 4) only a pair of counter-propagating beams. 


%  For $\sigma_+$-$\sigma_-$, 
% the atom-field interaction Hamiltonian for the counter-propagating beams is:
% \begin{equation}
%     H_{AF}^{\sigma_+-\sigma_-} = \sum_i \Omega_i  \left[ ( \hat{\mathcal{R}} \Sigma_{1}^\dag + e^{i \phi_i} \hat{\mathcal{R}}^\dag \Sigma_{-1}^\dag ) + h.c.   \right]
% \end{equation}
% We assume that the atom is situated around a position $z=0$, where it experiences linear polarization determined by the retro phases $\phi_1$ and $\phi_2$ for the two different frequencies.
% Since the cooling and repumper lights have different frequencies, their phase accumulation from the atom to the mirror and back differs by $\phi_{1/2} - \phi_{3/2} \approx 0.3 (2 \pi )$. All three retro mirrors are positioned about 10 inches away from the atoms. This phase difference results in the linearly polarized light seen by the atom at the two frequencies having different angles.  

% When the phase difference is zero, the two polarizations are linear and aligned. However, in our experiment and simulation, this phase seems to be of little importance, likely because the repumper has 10 times less power than the cooling beam and does not contribute significantly to the AC Stark shifts.

%  Performing the LD expansion of this atom-field Hamiltonian gives (for a single frequency)
%  % \begin{equation}
%  %     H_{AF}^{\sigma_+-\sigma_-} \approx \Omega_i \left[  \left( \Sigma_{1}^\dag  + e^{i \phi_1} \Sigma_{-1}^\dag \right) + i k  \hat{z} \left( \Sigma_{1}^\dag  - e^{i \phi_1} \Sigma_{-1}^\dag   \right) \right]
%  % \end{equation}
% In the LD regime, the zeroth order term does not couple different motional states $|n \rangle$, but does couple the levels within a single motional state and results in the dressed states shown in the cartoons of Fig.~4 in the main paper.  The first order term results in coupling between different motional states. 
% Interestingly, it is this sign difference in the zeroth order and first order term that allows the first order coupling term to mix bright and dark states of different $|n\rangle$.  Without that sign difference, the bright and dark states of neighboring $n$ would not be coupled. 

% %\subsubsection{Cross-coupling}
% The steady-state solver is unable to handle time-dependent interactions. Given that the cross-coupling is off-resonant, we assume that the scattering rate is small compared to that of the main beams. To address this, we derive additional effective cross-coupling collapse operators as follows:
% % \begin{equation}
% %     \hat{C}_i = \sqrt{\Gamma \frac{ \Omega_i^2}{4 \Delta_i^2}}  \left[  \Sigma_{1,i}^\dag \hat{\mathcal{R}} + e^{i \phi_i} \Sigma_{-1, i}^\dag \hat{\mathcal{R}}^\dag  \right]  
% % \end{equation}
% where $\Delta_i$ represents the detuning of the cross-coupling beams to the $F'=3/2$ excited state. These collapse operators are derived by first moving to a rotating frame of the cross-coupling beams, then transitioning to the dressed frame of the time-independent interaction, considering only first-order terms in saturation, and finally returning to the rotating frame of the main beams.

% The cross-couplings introduce additional AC Stark shifts, which might affect the $F=1/2$ and $F=3/2$ states. However, we find this impact to be minimal and thus ignore it. The primary effect is the introduction of new collapse operators that correspond to decay from the ground to excited state. These new collapse operators serve two purposes: 1) they induce recoil heating at the rate of off-resonant scattering of the cross-coupling beam, and 2) they cause mixing between the dark and bright states.

 
% For the 2D simulations shown in Fig.~4 of the main text, we get 
%  from 2d simulations in paper,  $T = 1.2 (hw/kBT)^-1$,  or  41 uK for radial,  $<n> = 3.0$
%  for axial 12,  or  82 uK.  $<n> = 5.0$
%  0.006 excited for both.  
% $(2*(<nradial> +1/2)*34uK + (<naxial>+1/2)*34/5 uK) = 3 kBT$,  or T = 92 uK. 


% \bibliography{apssamp}% Produces the bibliography via BibTeX.
% \bibliography{bibliography}



% Optical tweezers have typical waists less than a micron and trapping frequencies above 100 kHz, so well within the LD regime, although some species  are borderline  and require special treatment for higher $n$\cite{yu2018motional}.
% The Lamb-Dicke parameter can also be defined in terms of the recoil energy and the motional quanta i.e.  $\eta^2  = E_\text{recoil} / {\hbar \nu} $, where $E_\text{recoil} = \frac{\hbar^2 k^2}{2 m }$ is the average energy acquired from one recoil (note that actually recoil displaces momentum and creates a diffusion within n, so this is an averaged effect).  We can also think of the LD regime as when the recoil energy is smaller than the separation between $n$ states, and therefore one recoil most likely does not change the $n$.  

% Cooling is a balance between the direct coupling of neighboring motional states $|n\rangle$$\rightarrow$$|n-1 \rangle$ and the diffusion caused by recoil, which on average heats by $E_\text{recoil}$ per photon.  As shown in Fig.~\ref{fig:subdoppler_schematic}, the cooling can be described by a system of two internal state manipulating steps: the first step is optically pumping between electronic states $|1,n \rangle$$\rightarrow$$|2, n-1 \rangle$ followed by spontaneous emission back to the original electronic state $|1, n-1 \rangle$, which in the LD regime most likely doesn't change the motional state. 

% For neutral atoms, the linewidth, typically around 5 MHz, is generally larger than the trapping frequency, usually at around 100 KHz. This leads to an unresolved sideband regime where distinguishing between $n\rightarrow n-1$ and $n \rightarrow n$ can be challenging. However, narrow linewidth transitions on the order of $\sim$100 kHz, as seen in alkaline earth metals, can resolve them. Furthermore, it is essential for the excited state to have the same potential. This condition is often not met for neutral atoms, except at particular `magic' wavelengths. 

% We can make a quick estimate of the temperature by considering the cooling and scattering rates between different $n$ as shown in Fig.~\ref{PG_cooling_figure}.
% The population in $|e, n \rangle$ decays to different ground motional states with branching ratios in the LD regime  $\Gamma_{n \rightarrow n'}/(\sum_{m} \Gamma_{n \rightarrow m})  \approx |\langle n| \eta (\hat{a} + \hat{a}^\dag)|n' \rangle|^2 $ . % maybe put excact here
% From these we can derive a rate equation for the populations $P(n)$ in each $n$ state given by
% \begin{gather}
%     \frac{d}{dt}  P(n) = \Gamma_s \eta^2 \left[  -(2n+1) P(n) + (n+1) P(n+1) + n P(n-1)      \right] \nonumber \\
%     - R_{c}(n) P(n) + R_{c}(n+1) P(n+1)
% \end{gather}
% \Jon{what should $\Gamma_s$ be? I don't think I defined that. we need to make them consistent with figures as well.}  

% This is in the limit where the population is mostly in the ground state, spontaneous emission drives from $|e\rangle$ to $|g\rangle$ and no coherence is present between the ground states. Only then we can write it as a classical rate equation that includes the diffusion from scattering in the first term, and cooling in the second term. 
% We can also calculate the steady state average population $\langle n \rangle = \sum_{n=0}^\infty n P(n)$:
% \begin{equation}
%     \frac{d}{dt} \langle n \rangle = \Gamma_s \eta^2 - \langle R_{c}(n) \rangle
% \end{equation}
% where we can then see that the net effect of the recoil is an increase from $n$ to $n+1$ with rate $\Gamma_s$ $\eta^2$(n+1), which is consistent with $\eta^2 = E_\text{recoil} / \hbar \nu$.
% Another useful measure is the ratio of the ground state population to the first excited population, which is given by
% \begin{equation} \label{eq:P0P1}
%     \frac{P(n\!=\!0)}{P(n\!=\!1)} = \frac{\Gamma_s \eta^2 + R_{c}(n=1)}{\Gamma_s \eta^2 } = 1 + \frac{ R_{c}(n\!=\!1) }{\Gamma_s \eta^2}
% \end{equation}
% This derivation uses $R_{c}(n\!=\!0) = 0$ as there is no more state for it to couple to.  We can also make an estimate for the cooling rate $R_{c}(n)$ by considering the schematic in Fig~\ref{PG_cooling_figure}.  We have a coherent coupling $\Omega_{cool}$ and a pumping rate $\Gamma_{p}$, then the well-known scattering formula gives the overall transfer between $|1, n \rangle$ and $|1, n-1 \rangle$
% \begin{equation}  \label{eq:Rc}
%    R_{c}(n) = \frac{\Omega^2_{c}(n) / \Gamma_{p}}{1 + 2 \Omega_{c}^2(n)/\Gamma_{p}^2 + 4 (\delta - \nu)^2/\Gamma_{p}^2}
% \end{equation}

% This equation includes the saturation effect when the cooling rate is larger than the pumping rate, and when the 2-photon detuning is same as the vibrational frequency. This can be inferred directly from the typical scattering equation for a TLS.

% The criterion for optimum cooling is straightforward: in the dressed frame, the state $|2,n \rangle$ should be degenerate with $|1,n-1 \rangle$, indicating that the two-photon transition is resonant.
% Examining the last two equations, we can identify the two distinct cooling regimes, defined by whether the ratio $\Omega_{c}/\Gamma_{p}$ is greater than or less than one. In the regime where this ratio is less than one, we have $R_{c}(n) = \Omega^2(n)/\Gamma_{p}$. However, when the cooling rate increases beyond this point, it eventually reaches a saturation level, where $R_{c} \approx \Gamma_{p}/2$., in which case the ratio becomes:
% $P(n\!=\!0)/P(n\!=\!1) \approx  1 +  \frac{\Gamma_{p}}{2 \Gamma_s} \frac{1}{\eta^2}$. Then the temperature is just given by inverse squared of the LD parameter times the pumping rate over how dark the states are during the coherent transfer. Different sub-doppler cooling schemes lower the temperature further by making the dark state darker.  GM adds dark states that the polarization of light cannot couple to.  EIT creates a dark state as a antisymmetic superposition of two ground states that decouples it from the excited state.  Raman sideband cooling takes it to the extreme case by separating the repumper and coherent drive as separate beam so that the coherent transfer has negligible scattering and the repumper uses the minimum number of photon scattering.

% %%%%%%%%%%%%%%%%%%%%%%%%%%%%%%%%%%%%%%%%%%%%%%%%%%%%%%%%%%%%%%
% \subsection{dipole fluctuating force}
% Allow excited state to have different potential.
% Ref \cite{martinez2018state}
% Also look at Bernio paper. 


% %%%%%%%%%%%%%%%%%%%%%%%%%%%%%%%%%%%%%%%%%%%%%%%%%%%%%%%%%%%%%%%%%
% \newpage

% \subsection{Lambda-enhanced gray molasses}

% \subsubsection{Grey Molasses}
% Laser power and detuning dependence for specific trapping:


% For spsm and lin-per-lin both we get 0.986 GSP in the GM case, so max are identical. It is also interesting to see that if we compare PG cooling and Gm cooling, GM is much broad and cold compared to PG. Need to explain why.


% \subsubsection{Lambda enhancement}

% Till now we have talked about only a single laser and a fine structure atom. We are introducing hyperfine structure now for the first time. System is two ground states with one excited state and two spsm coherent lasers interacting with a bound atom.

% For optimum cooling the two neighboring hyperfine ground states (g1,g2) should be degenerate. This can be achieved by finding the balance between trapping frequency of the trapping laser and Rabi frequency of the cooling laser. The matching condition is introducing same vector shift by trapping laser as the tensor shift by the cooling laser.

% The condition for maximum ground state population, i.e., optimum cooling in case of Grey Molasses in Rb87 (single hyperfine excited), is given by the equation:


% \newpage

% Diiferent $\eta$ plots:


% Cooling Characterization at wh=0.01:





% \newpage




% \newpage 


% Here, we briefly review light shifts. The light shift between two levels $|J_g, m \rangle $ and $|J_e, m \rangle $  with detuning $\Delta$ is 
% \begin{equation}
%     \Delta E_{AC} = \sum_{m_e, q} \frac{|\langle J_g, m | E_q d_{-q}  | J_e, m\rangle |^2}{(\omega - \omega_{e})^2}  = |\langle J_g || d || J_e\rangle|^2  \frac{\langle J_g mg 1 q | J_e m_e \rangle^2  }{(\omega - \omega_{e})^2}
% \end{equation}
% It is proportional to the Clebsch-Gordon coefficients. Summing up all the contributions from the excited state gives an overall shift. 
% The overall shift for ground state $|J_g, m_g \rangle$ takes a convenient form in terms of the polarization of light when the tensor polarizability is separated into the scalar, vector, and tensor components:
% \begin{equation}
% \Delta E(m) = - \alpha_{0} |E|^2 - \alpha_{1}  \left( |E_{1}|^2 - |E_{-1}|^2\right)  \frac{m}{J}  - \alpha_{2}  \frac{ \left(3 |E_z|^2 - |E|^2  \right)}{2}  \left( \frac{3 m^2 - J(J+1)}{J(2J-1)}  \right),
% \end{equation}
% The scalar shift depends only on the electric field's magnitude and shifts all states the same amount. The vector components shift is proportional to $m$ just as a B field depends on the ellipticity of light and is often called an artificial B-field. The tensor components are related to how aligned the polarization is with the quantization axis and is maximum when the polarization is along $\hat{z}$ and minimum when no components are along $z$.    

% OLD: Now in this form, we can easily see the effects of the polarizations in the two PG cases. 
% There is no vector shift in the $\sigma_+-\sigma_-$ configuration since the light is linear everywhere, and the tensor shift becomes the dominant contribution.    We need at least three ground states to observe PG cooling, and also it needs to have comparable tensor shift( $\sigma_+-\sigma_-$) and vector shift(LinLin) so we chose $J=2$ to $J=3$ for our simulation. We will later see that $J=1$ to $J=1$ or $J=0$ is dominated by GM effects.


% %The scalar, vector, and tensor polarizabilities all are similar in magnitude when close to hyperfine states. As the detuning is increased compared to the hyperfine splittings, then the tensor shifts get cancellation between the different excited hyperfine states and diminish. When the detuning is large compared to the fine structure, the vector shift also deconstructively interferes.  
% %However, this tensor shift will get smaller as the light couples to multiple excited hyperfine states. 


% We consider the first term in the interaction that does not change $n$, only the diagonal components of $\langle n | \mathcal{R} | n \rangle$. Looking first at $\sigma_+-\sigma_-$, that is just linear light. Detuned from the excited state by $\Delta$, this light will cause a tensor shift, as shown in Fig.~\ref{PG_cooling_figure}. The scattering will also optically pump the population.   For linear light and $J_e' \ge J_g$, the population accumulates in the $m_g=0$ state, as one might expect linear light to result in a linear steady-state polarization. However, for the case of $J_e' < J_g $, the stretch states are dark, and the populations accumulate in these dark states.   For $J_g=1$ to $J_e=2$, the AC stark shifts and populations 
% are shown in Fig.\ref{PG_cooling_figure}. One criterion for cooling with light shifts is that the population accumulates in the lower-energy state. We also introduce an optical pumping rate from the higher energy to lower energy state $\gamma_p$, which will be similar to the scattering case since it only takes a few scattered photons to go $m=0$. 

% The $n$ changing interaction  $\eta(a + a^\dag) \Sigma_x^\dag$ drives the orthogonal polarization.   In Fig.~\ref{PG_cooling_figure}, we draw the neighboring states. The role of this interaction is to play the second branch of the two-photon transitions, which are shown with blue arrows.   The two-photon transition is resonant when the differential AC Stark shift equals the trapping frequency $\nu$.    Interestingly, if the two beams were co-propagating (same k-vector), this term would also be $\Sigma_0$, and there would be no coupling. So we can see in this framework that the role of the k-vector is making the atom excitation of the LD term orthogonal to the 0th order term to couple different states in different $n$. 

% \cite{Wineland1992Sisyphus, GBirkl1994Polarization}



% \vspace{30 mm}
%  This cooling metric is more straightforward to calculate than, for example, $\langle n\rangle$ because the rate equations are not in general linear with $n$.  There is a two-photon transition for PG cooling between $|g_1, n \rangle $ and $|g_2, n \rangle$.  Therefore both $A_{00} = A_{11} = 0$, which interestingly was not the case for RSB.  % The $A_{n,n}$ terms are zero because the linear zeroth order term cannot coherently transfer from $|m=0 \rangle$ to $|m=\pm1 \rangle$. 
% The cooling metric is then
% %
% \begin{equation}
%     \frac{P(0)}{P(1)} = \frac{A_{1,0} + \eta^2 \gamma_s  }{  A_{0,1} + \eta^2 \gamma_s}
% \end{equation}
% %
% where $A_{1,0}$ is the rate at which you drive $n=1$ to $n=0$ (which is two-photon resonant) and $A_{0,1}$ is the rate at which you drive $n=0$ is to $n=1$ is which is two-photon detuned by $\delta = 2 \nu$.  The scattering rate $\gamma_s$ is the off-resonant scattering rate when the population is optically pumped into a steady state ground state.  We define a coefficient $c_s$ 
%  such that $\gamma_s = c_s \Gamma \Omega^2/\Delta^2$.


% First, we look at the cooling rate $A_{1,0}$.   When the differential light shift equals the trapping frequency, $\delta_{AC} = \nu$, this process is two-photon resonant, and is given by
% %
% \begin{equation}  
%     A_{1,0} = \gamma_p \frac{ (\Omega_{R}/\gamma_p)^2}{ 1 + 2 (\Omega_{R}/\gamma_p)^2  }
% \end{equation}
% %
% $\Omega_R$ is defined in Eq. and is approximately $c_R  \Omega^2/\Delta$. 
% The off-resonant scattering/pumping rate $\gamma_p$ is the rate at which $g_1$ pumps to $g_2$.  Because the $\gamma_p$ scales with $1/\Delta^2$ and $\Omega_R$ with $1/\Delta$, the detuning can be increased enough to saturate the cooling process, in which case 
% %
% \begin{equation}
%  A_{1,0} \approx \gamma_p/2   \quad \text{for $\Delta/\Gamma \gg$ 1 }
% \end{equation}
% %
% Next, we look at the heating rate $A_{0,1}$, which takes a similar form except because it is off-resonant by $\delta = 2 \nu$, need to include the detuning   %The rates $A_{1,0}$ and both contain $\Omega_{1,0} = \Omega_{0,1} = \Omega_R $. 
% \begin{equation}  \label{eq:Ann}
%     A_{0,1} = \gamma_p \frac{ (\Omega_{R}/\gamma_p)^2}{ 1 + 2 (\Omega_{R}/\gamma_p)^2 + 4 (2\nu /\gamma_p)^2  }
% \end{equation}

% In the cooling metric, we can ignore $A{0,1}$ when it is small compared to $\eta^2 \gamma_s$.  This ratio is $A_{0,1}/\eta^2\gamma_s \approx 1/16 \gamma_p/\gamma_s  \alpha_R^2/\alpha_2^2$ is generally less than 1.  
% %$\Delta E_{AC}(m=1) -\Delta E_{AC}(m=0)  = \alpha_{(2)} \Omega^2/\Delta$
% Then the cooling metric becomes
% \begin{equation}
% \frac{P(0)}{P(1)} \approx 1 + \frac{A_{1,0}}{\gamma_s \eta^2} = 1 + \frac{1}{2 \eta^2} \frac{\gamma_p}{\gamma_s}.
% \end{equation}
% The cooling depends on two factors.  First, it improves with a smaller LD parameter as $1/\eta^2$.  However, it also depends on the ratio of the off-resonant scattering rate that pumps the population $\gamma_p$ to the off-resonant scattering rate of the pumped (steady-state population in $|g_2, 0 \rangle$) $\gamma_s$.  The darker the lower energy state, the lower temperature. 

% This principle motivates the two other forms of cooling we look at GM, which make the state darker by using polarization selection rules.



% The major limitation of PG cooling is that the lower energy state has just as much scattering as the higher energy states.   Gray molasses takes advantage of the dark states due to angular momentum selection rules when $J_e \le J_g$.   If $J_e = J_g$, a dark state exists for circular polarization.  However, for $J_e < J_g$, any polarization has a dark state.  Because we found for PG cooling that the cooling metric depends on the ratio of dark scattering rate to pumping rate,  Gray-Molasses can achieve much colder temperatures in principle.   However, because the lower energy state must be the one that is pumped to, GM requires blue-detuned light so that the AC Stark shift of the non-dark states is positive, and the dark state is the lowest energy. 

% The criteria for GM cooling when $\delta_{AC} \approx \nu$. , but because the dark states are not shifted, $\delta_{AC}$ is larger meaning that requires more power to compensate with $\Omega^2/\Delta$, or more power for a given detuning.  

% The pumped state is perfectly dark when the polarization is perfectly linear.  Setting $\gamma_s=0$ in the cooling metric gives
% \begin{equation}
%     \frac{P(0)}{P(1)} \approx \frac{A_{1,0}}{A_{0,1}}
% \end{equation}
% which shows that the cooling for GM, after we have added a dark state, is determined now not by the ratio of cooling to off-resonant scattering but by the ratio of cooling (which is resonant) to heating (which is off-resonant by $2\nu$). 

% \begin{equation}
%     \frac{P(0)}{P(1)} \approx \frac{A_{1,0}}{A_{0,1}} =  \frac{8}{ \eta^2} \left(\frac{ \alpha_{GM}}{\alpha_R}\right)^2
% \end{equation}
% It still depends on $1/\eta^2$, but now the temperature is set by how far apart the states are light shifted relative to the entire shift.  Because the vector shift is usually larger than the tensor shift for close detunings, that suggests lin$\perp$lin will have colder temperatures. 


% %%%%%%%%%%%%%%%%%%%%%%%%%%%%%%%%%%%%%%%%%%%





% degenerate raman sideband cooling?

% "adiabatic elimination slaves rapidly oscillating excited amplitude to the slowly varying ground state"
% \begin{equation}
% H_I^{\text{eff}} = \frac{1}{4} \bm{E}^*(\hat{x}) \cdot \boldsymbol{\alpha} \cdot \bm{E}(\hat{x}), \quad  =  -\frac{1}{4} E^*_j(\hat{x}) E_k(\hat{x}) \alpha_{jk}
% \end{equation}
% $\bm{E}(\hat{x}) =  E_0  \,  \hat{\epsilon}(\hat{x})    $

% \begin{equation}
% \boldsymbol{\alpha} = \sum_{F,F'} \frac{P_{g,F} \bm{d} P_{e,F'}  \bm{d} P_{g,F} }{\hbar(\Delta_{F'F} + i \Gamma / 2)}
% \end{equation}

% \begin{equation}
%     H_{\text{eff}}^I = -\frac{1}{4} E_j E_k \alpha_{jk}, \quad \alpha' = -\frac{1}{\hbar} \sum_{F'} \frac{\bm{d}_{FF'} \bm{d}_{F'F}}{\Delta_{FF'} + i \frac{\Gamma}{2}},
% \end{equation}

% \begin{gather}
%     \hat{D}^{\dagger}_{F'F} \equiv \frac{  P_{e,F'} \bm{d} P_{g,F}  }{\langle nP_J || d || nS_J \rangle} \\
%     = \sum_{q,M,M'} \bm{e}^{*}_q \,\,  o^{J'F'}_{JF} \langle F' M'  | F M ; 1 q \rangle \,\,
%       | F' M' \rangle \langle F M |
% \end{gather}


% \begin{equation}
%     o^{J'F'}_{JF} = (-1)^{F+1+J'+I} \sqrt{(2J' + 1)(2F + 1)}
%     \left\{
%     \begin{array}{ccc}
%     F' & I & J' \\
%     J & 1 & F
%     \end{array}
%     \right\}
% \end{equation}


% collapse operator
% \begin{equation}
%     W_q = \sum_{F'} \frac{\Omega/2}{\Delta_{FF'} + i \Gamma/2} \left( \bm{e}_q^* \cdot \bm{D}_{FF'} \right) \left( \bm{\hat{\epsilon}} \cdot \bm{D}_{F'F}^\dag \right).
% \end{equation}

% \begin{equation}
%     \frac{d\rho}{dt} = \frac{i}{\hbar} \left( H_{\text{eff}}^A \rho - \rho H_{\text{eff}}^{A \dagger} \right) + \Gamma \sum_q W_q \rho W_q^\dagger,
% \end{equation}

% \begin{gather}
%     \gamma_{FM_1 \rightarrow FM_2} = \sum_{q} \left| \langle F{M_2} | W_{q} | F{M_1} \rangle \right|^2 \nonumber \\
%     % = \frac{\Omega^2 \Gamma}{4} \sum_{q} \Biggl| \sum_{F'} \frac{\langle F{M_2} | \left( \bm{e}_q^* \cdot \bm{D}_{FF'} \right) \left( \bm{\hat{\epsilon}} \cdot \bm{D}_{F'F}^\dag \right) | F{M_1} \rangle}{\Delta_{FF'} + i\Gamma/2} \Biggr|^2,
% \end{gather}

% \begin{gather}
%     H_{I,\text{eff}}  =  V_0 \Bigl[ C_{J'F'F}^{(0)}     |\boldsymbol{\varepsilon}|^2 %\nonumber \\
%     + i C_{J'F'F}^{(1)} (\boldsymbol{\varepsilon}^* \times \boldsymbol{\varepsilon}) \cdot \bm{F} \nonumber \\
%      + C_{J'F'F}^{(2)} \left(|\boldsymbol{\varepsilon} \cdot \bm{F}|^2 - \frac{1}{3} \bm{F}^2 |\boldsymbol{\varepsilon}|^2 \right) \Bigr],
% \end{gather}
% where
% $ |\boldsymbol{\varepsilon} \cdot \bm{F}|^2 = \frac{1}{2} \left[ (\boldsymbol{\varepsilon} \cdot \bm{F})^\dag (\boldsymbol{\varepsilon} \cdot \bm{F}) + (\boldsymbol{\varepsilon} \cdot \bm{F})(\boldsymbol{\varepsilon} \cdot \bm{F})^\dag \right].$
% \begin{equation}
%     V_0 = \frac{1}{4} \alpha_0 |E_0|^2 = \frac{\hbar \Omega^2}{4 \Delta_{\text{FF}}} = \left( \frac{\hbar \Gamma I}{8 I_{\text{sat}}} \right) \frac{\Gamma}{\Delta_{\text{FF}}},
% \end{equation}






% From above:
%  and the normalized dipole lowering operator expanded in terms of the spherical unit vectors
% \begin{equation}
% \bm{D} =  |o_{JF}^{J'F'} | \sum_{q, m_e, m}  {\hat{\bm{e}}}^*_q \, \langle F m ; 1 q | F m \rangle  \,\,   | F m \rangle \langle F_e m_e|
% \end{equation}  % CHECK THESE.  
% or
% \begin{equation}
% {D_q} = |o_{JF}^{J'F'} | \sum_{m_e, m} \langle F m ; 1 q | F m \rangle  \,\,   | F m \rangle \langle F_e m_e|
% \end{equation}  % CHECK THESE.  
% where $o_{JF}^{J'F'}$ is the oscillator strength of the transition

% \[
% o_{JF}^{J'F'} = (-1)^{F+1+J+I} \sqrt{(2J' + 1)(2F + 1)}
% \begin{Bmatrix}
% F' & I & J' \\
% J & 1 & F
% \end{Bmatrix}
% \]


% While the dipole operator $d_q$ is a spherical vector operator, $\Sigma_q$ is not. For example $(\Sigma_q)^\dag \ne  (\Sigma_{-q})$.

% With this formalism, the interaction Hamiltonian is 
% \begin{equation}
% H_{\text{I}} = \frac{\hbar}{2} \sum_q \left[  \Omega_{q} (\hat{z}) \, \Sigma^\dag_{q} \,   + \,h.c.   \right],
% \end{equation}
% where the Rabi frequencies are defined in terms of the reduced matrix elements
% \begin{equation}
% \Omega_{q}(\hat{z}) = - \frac{2}{\hbar}  \langle J_g || \bm{d} || J_e \rangle   \, \mathcal{E}^{(+)}_{q}(\hat{z}).
% \end{equation}

% The repopulation of the ground state comes from six collapse operators corresponding to an emission of a photon with polarization $q$ in either the forward or backward direction
% \begin{equation}
%  \hat{C}_q =  \sqrt{\Gamma} \, {\Sigma}_q e^{\pm i k \hat{z}}
% \end{equation}


% \begin{equation}
%     \boldsymbol{D} =  \frac{P_{g,F_g} \boldsymbol{d} P_{e,F_e} }{\langle J_e || d ||  J_g\rangle  },  \quad \boldsymbol{D}^\dag =  \frac{P_{e,F_e} \boldsymbol{d} P_{g,F_g} }{\langle J_e || d ||  J_g\rangle  }.   % which order should I put this? Steck is J  J'
% \end{equation}
% \begin{equation}
% H_0 =  \sum_{m_g}  \hbar  \Delta  \, |F_g, m_g \rangle \langle F_g, m_g| + \hbar \nu a^\dag a . 
% \end{equation}
% The excited states $|F_e, m_F \rangle$ are defined as zero energy, which is why they do not appear in the Hamiltonian. 

% We write the complex electric field as the sum of plane waves with wave vectors $\bm{k}_j$
% \begin{equation}
% \mathcal{E}_q^{(+)}(\bm{r}) =\frac{1}{2} \sum_j  \mathcal{E}_{j,q} e^{i \bm{k}_{j} \cdot \bm{r}}.
% \end{equation}
% where $E_{q,j}$ are the polarization in the $q$ component of the $j$' th  beam, and the position in the phase is promoted to a quantum operator. 

% \begin{gather}
% H = \nu a^\dag a  +   \left( \Delta - i \frac{\Gamma}{2} \right) P_e  - \frac{\Omega}{2}  \left( \boldsymbol{\mathcal{\epsilon}}(\hat{x} ) \cdot \boldsymbol{D}^\dag + h.c. \right).
% \end{gather}

% \subsubsection{$\sigma_+ - \sigma_- $, Left-hand and right-hand polarization }

% The atom-field interaction is 
% \begin{equation}
% H_{I}^{\sigma_+-\sigma_-} = \frac{\Omega}{2} \left[ ( e^{- i k \hat{z}} \Sigma_{1}^\dag + e^{i \phi} e^{i k \hat{z}} \Sigma_{-1}^\dag ) + h.c. \right].
% \end{equation}
% where $\Omega = - \frac{2}{\hbar}  \langle J_g || \bm{d} || J_e \rangle   \, \mathcal{E}_0$.

% \begin{equation}
% H_{AF}^{\text{lin} \perp \text{lin}} = \frac{\Omega}{2} \left[ (\Sigma_{x}^\dag + e^{i\phi} \Sigma_{y}^\dag) + \eta(a+a^\dag) (\Sigma_{x}^\dag - e^{i\phi} \Sigma_{y}^\dag) + h.c. \right],
% \end{equation}

% ~\cite{steck}:
% \begin{equation}
% d_q = \langle J_g || d || J_e \rangle \left(\Sigma_q + (-1)^q \Sigma_{-q}^\dag \right) = d_q^{(+)} + d_q^{(-)}.
% \end{equation}

% The raising operators $\sigma^\dag$ of the two-level system are replaced with collective raising operators $\Sigma_q^\dag$ that create an excited state with one additional angular momentum $m_e = m_g + q$, 

% We will now compare our results with the case of Doppler cooling using a retro beam. In this case, the interaction Hamiltonian includes two recoil terms, one of which carries a phase: $e^{ikx} + e^{i \phi} e^{-ikx}$. This introduces an additional variable that can be experimentally adjusted, as the phase can be easily changed by modifying the spatial separation along the beam path to the retro mirror.



% Population in the harmonic potential states are redistributed by the laser detuned by $\Delta$ and the subsequent recoil from the spontaneous emission.  If the laser is detuned by $\Delta = - \nu $, it can preferentially drive $n \rightarrow n-1$, removing $\hbar \nu$ of energy at the scattering rate $A_-$, leading to cooling $\frac{dE}{dt} = \hbar \nu (- A_- + A_+)$.  Each spontaneously emitted photon removes $\hbar k$, however, the direction is random and the atom's momentum experiences a random walk and difussion. In a diffusion process, the momentum squared, or kinetic energy, increases linearly as $ \frac{dE}{dt} =  E_R \gamma_\text{s} $. 

% A similar result can be derived more formally by considering the scattering processes and the population rate equation. The Rabi frequency between state $n$ and $n'$  is $\Omega_{n \rightarrow n'} = \Omega_0  \langle  n | e^{-i k z} |n' \rangle $. In the low saturation limit, the scattering rate between two-levels with Rabi frequency $\Omega$, detuning $\Delta$, and excited state decay $\Gamma$ is total rate $\gamma(\Delta) P(n)$, where
% \begin{equation}
%     \gamma(\Delta) =  \frac{\Omega_{n,n'}^2}{\Gamma} \left( \frac{1}{1 + 4 \Delta^2/\Gamma^2 + 2 \Omega_{n,n'}^2/\Gamma^2} \right) .  
% \end{equation}  
% The excited state $n$ decays to different motional states by $\Gamma_{n\rightarrow n'} = \Gamma |\langle  n | e^{-i k z} |n' \rangle |^2 $. 

% Defining a TLS scattering rate (non-saturating)
% \begin{equation}
%      \gamma(\Delta) =  \frac{\Omega^2}{\Gamma} \left( \frac{1}{1 + \Delta^2/(\Gamma/2)^2 } \right) .  
% \end{equation}

% The non-interacting Hamiltonian for a two-level system emitter in a harmonic potential in the rotating frame of the laser with $\Delta = \omega_A - \omega_L$ is 
% % \begin{equation} \label{eq:H0}
% %     H_0 = \left(\Delta -  i \frac{\Gamma}{2}\right)  |e \rangle \langle e | + \nu \hat{a}^\dag \hat{a} %\frac{\hat{\bm{p}}^2}{2 m} +  \frac{1}{2} m \nu^2 \hat{z}^2  .
% % \end{equation}

% The complex field ${\boldsymbol{\mathcal{E}}}(\hat{z})$ contains the polarization and the position operator. %, and is related to the electric field amplitude by  
% The interaction of the atom with the field in the rotating frame of the laser is 
% % \begin{equation}
% %     H_{I} = \bm{d} \cdot \bm{\mathcal{E}}^{(+)}(\hat{z})  \, \hat{\sigma}^\dag + h.c. ,
% % \end{equation}
% \begin{equation}
%     H_{I} = \frac{\hbar}{2} \Omega(\hat{z}) \, \hat{\sigma}^\dag + h.c. ,
% \end{equation}
% where
% \begin{equation}
% \Omega(\hat{z}) = -2 \frac{1}{\hbar}  \langle g | \bm{d} | e \rangle   \cdot \bm{\mathcal{E}}^{(+)}(\hat{z}).
% \end{equation}
% Here $\bm{d}$ is the atomic dipole operator,, and the time dependence of the electric field is cancelled out in the rotating frame of the laser. 

% The basis of the non-interacting Hamiltonian are the ground states $|g, n \rangle$ and excited states $ |e, n' \rangle$.  In this basis, the laser drives transitions $|g, n \rangle \rightarrow |e, n' \rangle$.  
% The interaction produces a coupling between states $|g, n \rangle$ and $|e, n' \rangle $ with Rabi frequencies
% \begin{equation}
%     \Omega_{n,n'} =  \langle g,n| \Omega(\hat{z}) \sigma |e, n' \rangle =  \langle n| \Omega(\hat{z}) | n' \rangle 
% \end{equation}
% In this quantized picture, the laser cools by driving $|g, n \rangle \rightarrow |e, n-1 \rangle$, which occurs at a detuning of $\Delta = -\nu$.

% For a single plane wave, %$\mathcal{E}^{(+)}(\hat{z}) =  \mathcal{E}_0 e^{ik\hat{z}}$. 
% $\Omega(\hat{z}) = \Omega_0 e^{ i k \hat{z}}$.  Because this has the same form as the recoil operator, we can interpret this position dependence as the recoil due to photon absorption. The Rabi frequencies between different motional states are
% \begin{equation}
%     \Omega_{n,n'} = \Omega_0 \langle n | e^{- i k \hat{z}} | n' \rangle. 
% \end{equation}  % should this be positive

% In the LD regime, the only couplings are  $\Omega_{n,n} = \Omega_0$, $\Omega_{n,n+1}=  \sqrt{n+1} \, \eta \Omega_0 $ and $\Omega_{n,n-1} =  \sqrt{n} \, \eta \Omega_0$. These are shown in Fig.~\ref{fig:Doppler}(b).  

% The $|e, n \rangle$ population decays into different motional states with rates
% \begin{equation}
%     \Gamma_{n \rightarrow n'} = \frac{\Gamma}{2} \sum_{\pm} |\langle n | e^{\pm i kz} |  n' \rangle|^2 =\Gamma \, |\langle n | e^{i kz} |  n' \rangle|^2 
% \end{equation}

% The total deacy  of excited state in state $n$ is $\Gamma =\sum_{m} \Gamma_{n \rightarrow m}$. % the branching ratio is given by
% the LD regime  $\Gamma_{n \rightarrow n'}/(\sum_{m} \Gamma_{n \rightarrow m})  \approx |\langle n| \eta (\hat{a} + \hat{a}^\dag)|n' \rangle|^2 $ .  Shown in 

% The total Hamiltonian for a two-level system in a harmonic trap with one plane wave is 
% \begin{equation}
%     H =  \left(\Delta - i \frac{\Gamma}{2}\right) | e \rangle \langle e | + \nu a^\dag a + \frac{\Omega_0}{2} \left( e^{- i k \hat{z}} \hat{\sigma}^\dag + h.c.  \right),
% \end{equation}
% with again collapse operators $\hat{C}_\pm =  \hat{\sigma} e^{\pm i k \hat{z}} $ to repopulate the ground state. 


% We can estimate the ground state population by creating a population rate equation.
% We will assume below saturation so atom is mostly in ground state.  Defining the population in ground state $n$ as $P(n)$, we can the decay rate between different states.  This can be derived formally from the optical Bloch equations by eliminiating the excited state and settings the coherences between motionatl states to zero, which is justified because the sponatneous emission results in loss of coherenc  between different $n$ in the ground states.  
% In the LD approximation, keeping all first order terms, the scattering rate out of state $P(n)$ is 
% %
% \begin{gather}
%     \frac{d P(n)}{d t} =  \eta^2 \biggl[ P(n) \biggl\{ -(2 n + 1) \gamma(\Delta) \nonumber \\
%     +  (n+1) \gamma(\Delta + \nu) +  n \gamma(\Delta - \nu)  \biggr\} \nonumber \\
%     + (n+1)  P(n+1)\biggl\{ \gamma(\Delta-\nu) + \gamma(\Delta) \biggr\} \nonumber \\
%     +n P(n-1)  \biggl\{ \gamma(\Delta + \nu) +  \gamma(\Delta)\biggr\}   \biggr]
% \end{gather}
% %
% The rate equation shows the diffusion of the population due to scattering. 
% The $\eta^2$ appears because it is the ratio of the recoil energy to the vibrational quanta. By multiplying both sides by $n$ and summing over all $n$, we can calculate the time evolution for $\langle n \rangle = \sum_n n P(n)$ 
% %
% \begin{equation}
%    \frac{d}{dt} \langle n\rangle  = \eta^2 \left[ \gamma(\Delta) +  (\langle n\rangle +1) \gamma(\Delta+\nu)  - \langle n \rangle \gamma(\Delta - \nu) \right].
% \end{equation}
% %
% This equation leads to a steady-state solution
% \begin{equation}
%     \langle n \rangle_\text{ss}= \frac{R(\Delta) + R(\Delta + \nu)}{R(\Delta - \nu) - R(\Delta + \nu)}
% \end{equation}
% %
% Because each term is proportional to the scattering, the power dependence cancels out in the unsaturated limit of $ 2\Omega^2/\Gamma \ll 1$. The steady state is insensitive to both power and $\eta$. It is also independent of $\eta$ as long as it is much smaller than 1, and the cooling will become less efficient for any higher $\eta$ values, as it is outside the LD approximation regime.

% In the resolved sideband regime, where $\nu > \Gamma$, the minimum temperature is
% %
% \begin{equation}
%     \langle n\rangle_\text{resolved} \approx  \frac{1}{1 + 4 \nu^2 / \Gamma^2}
% \end{equation} 
% which occurs at $\Delta \approx - \nu$.   The average energy decreases as $\Gamma/4 \nu^2 $ as the transition becomes more resolved. 

% The energy is higher in the unresolved sideband limit ($ \nu < \Gamma$) and converges to the Doppler temperature in the limit of small $\nu/\Gamma$ 
% \begin{equation}
%     \langle n\rangle_\text{unresolved}  \approx \frac{\Gamma}{2 \nu}  = \frac{ k_B T_\text{Doppler}}{ \hbar \nu}  . % CHECK THIS!
% \end{equation}
% As quote in previous results, the maxima is at a detuning $\Delta \approx -\Gamma/2$, but there is practically little difference between $\Gamma$ as seen in the simulation in Fig.~\ref{fig:Doppler}(c).
 
% The excited state potential is important because Doppler cooling operates close to resonance. We will first treat the case where the ground and excited have the same trapping frequencies, known as the magic condition. This special condition requires a specific wavelength or polarization with neutral atoms. Later, we will look at different potentials.   Trapping frequencies for netural atoms typically 100~kHz, whereas the linewidths is 5~MHz, so typcailly unresolved. Although narrow lines in alkaline-erath atoms are comparable. 

% how are atoms different from ions?
% For an atom in the tweezer, the depth of its trapping depends on two factors: the polarizability of the atomic state and the electric field of the trapping laser. Unlike ions, atoms can have a mismatch in the potentials between the ground and excited states due to different polarizabilities of the two. The excited state potential is especially important in Doppler cooling as it operates close to resonance compared to sub-doppler methods. Even when considering the simplest case of a a two-level atom, it is necessary to consider three distinct regimes: the polarizability of the excited state can be more, less, or equal to that of the ground state.


% Without resorting to spin and other polarization, Doppler cooling can be improved by intefering a counter-propagating beam, $\Omega(z) = \Omega ( e^{i k z} + e^{i \phi} e^{-ikz} )   )  $.   The phase of the counter-propagating beam determines where the atom is in the standing wave.  In Fig.~\ref{fig:Doppler}(f) we simulate the ground state fraction as a function of $\phi$.  Interestly, when the atom is at the node, the atom sees no intensity except when it oscillates  and the interaction is   $\mathcal{R} + e^{i \phi} \mathcal{R}^\dag \approx  2 i \eta (a^\dag + a) $  when atom placed at node.  and $e^{i \phi} = -1$.  Then $n \rightarrow n $ transition is not driven.  The ground state fraction is improved by a factor of four typically, but then the phase of the return beam needs to be controlled.



% Outside of LD regime, still has analytical solution solution~\cite{}
% \begin{equation}
% \langle n| e^{i k z} | n' \rangle = e^{-\eta^2} \left[ \frac{n_<!}{n_>!} \eta^{|n - n'|} L_{n_<}^{|n - n'|}\left(\eta^2\right) \right],
%    % check this with Wineland expression which also includes sign term, Experimental Issues in Coherent Quantum-State Manipulation of Trapped Atomic Ion 1998    
% \end{equation}
% where \( n_< \) and \( n_> \) are the lesser and greater of \( n \) and \( n' \), and \( L_k^{\alpha}(x) \) is the generalized Laguerre polynomial. hnhjg[i]poh h  j huikvn,uivygju21mc jqik


% The steady-state solutions are found using QuTip to solve for the steady-state solution of the full master equation~\cite{johansson2012qutip}. All the simulations done in this paper follow the same procedure.

% For approximate temperatures, we will further simplify the model.  Cooling usually takes place at low saturation and small excited state population.  Spin cooling like GM, PG, and RsB have even larger detuning.  In most cases, the excited state can be adiabatically eliminated.  The excited state is solved for in terms of the ground state and substituted in the ground state functions.  The exicted state population is slaved to the ground state population.\cite{deutsch2010quantum, reiter2012effective} % sorecnsen paper
%  % Deutsch and Jessen that I used a lot. mostly just appenix. 
% We will use this to create analytical  estimate for temperatures. 

% The spin dynamics can be further simplied into tensor operators by formalism in Ref.~\cite{deutsch2010quantum}.



% For the simulations, the LD regime is not assume.  The steady-state solution is found using the steady-state solver either found interatively or exactly depending the system size.  The number of harmonic states go up to 14.  


% \vspace{30mm}

% The bare Hamiltonian for a TLS in a harmonic potential is $H_0 = \Delta |e \rangle \langle e | + \nu a^\dag a $, and the interaction in the LD regime is approximated by 
% \begin{align}
%     H_{AF} &= \frac{\Omega}{2} ( \sigma^\dag e^{- i k \hat{z}} + h.c.)  \\
%     &\approx  \frac{\Omega}{2} ( \sigma^\dag + i \eta ( a^\dag + a) \sigma^\dag  + h.c. )
% \end{align}
% In this form, it is clear that the zeroth-order term does not change $n$, and the first-order term changes $n$ by $\pm1$. 

% The fundamental principle of laser cooling in a harmonic trap is how well one can resolve and drive $|n \rangle \rightarrow |n -1 \rangle$ and how well recoil heating can be minimized from spontaneous emissions during the cooling cycle.   These two principles are readily observed in a single-photon cooling scheme, such as Doppler cooling, as shown in Fig. ~\ref{Doppler_cooling_figure}. Detuning the laser from the transition by $\nu$ drives  $|g,n\rangle  \rightarrow |e,n-1\rangle$, which then decays mainly to $|g,n-1 \rangle$ when $\eta < 1 $ after spontaneous emission, resulting in a net cooling after one cycle if $\hbar \nu > E_\text{recoil}$.

% Polarization Gradient (PG), Gray Molasses (GM), $\Lambda$-enhanced GM, Electromagnetically Induced Transparency (EIT), and Raman Sideband Cooling (RSB) are all two-photon cooling schemes used in tight optical traps that increase $\Delta > \Gamma, \nu $ to selectively drive the red ground state motional sideband. As shown in the figure \ref{PG_cooling_figure}, there are two ground states $|g_1, n \rangle $ and $|g_2, n' \rangle $.

% The Hamiltonians for each scheme take the general form (in the rotating frame, with the excited state defined as zero energy)  $ H = \Delta_1 |g_1 \rangle \langle g_1 |  + \Delta_2 |g_2 \rangle \langle g_2 | +  \nu a^\dag a$  and interaction
% %
% \begin{equation}
%    H_{AF} =   \frac{\Omega}{2} \left[ \sigma_1^\dag e^{i k_1 \hat{z}} + \sigma_2^\dag e^{i k_2 \hat{z}} + h.c.  \right]
% \end{equation}
% %
% or in the LD regime, assuming counter-propagating beams with $k_2 \approx - k_1$, 
% %
% \begin{equation}
%   H_{AF}  \approx  \frac{ \Omega}{2} \left[ (\sigma_1^\dag + \sigma_2^\dag) + i \eta (a + a^\dag) ( \sigma_1^\dag - \sigma_2^\dag) + h.c.  \right]
% \end{equation}
% %
% The first term gives one branch of the two-photon transition, and the second term is the other branch, which also changes the motional state by $\pm 1$. 

% For two-photon cooling, the cooling criteria were similar to those for the single-photon scheme. How well can you selectively coherently drive $|g_1, n \rangle$ to $|g_2, n-1 \rangle$, and how few photons can you spontaneously emit during the transfer or while the atom is in $|g_2 \rangle$? 
% However, you can ask why we need many sub-Doppler cooling schemes such as PG, GM, $\Lambda$-GM, EIT, and RSB. What are the fundamental cooling limits for each system? Which is best for imaging? The schemes use different techniques for making the two-photon transition resonant, for optical pumping, and for making the ground state as dark as possible. For example, RSB usually performs best as it operates in the limit of $\Delta \gg \Gamma, \nu$ with negligible spontaneous emission and a separate near-resonant optical pumping beam.   However, requiring new lasers and several new beam paths is experimentally challenging. PG and GM use a single frequency with light shifts to make the $|g_1, n \rangle \rightarrow |g_2, n-1 \rangle $ transition resonant and the same light for optical pumping. EIT and $\Lambda$-GM are related, although they also use angular momentum selection rules or the dark states of a 3-level system to minimize scattering. Here 
% In this study,  we unite all these schemes into the same framework, calculate their properties, and compare them to simulations. 



% \Saumitra{For any quantum simulation experiment using tweezers, the first essential step is to achieve motional ground state population by cooling the single atom at each site using single photon or two photon processes. Despite the established understanding of sub-Doppler cooling techniques like Polarization Gradient (PG) and Gray Molasses (GM) cooling in free space, their efficacy in tight traps and the quantum descriptions of these processes remain less explored. This is especially relevant to the case of neutral atoms, where it is not uncommon for the ground and excited states to have different polarizabilities. For instance, what are the coldest temperatures you can achieve using these methods and what are their theoretical limits? What is the mechanism behind GM cooling that results in significantly colder temperatures compared to PG cooling? While choosing among various cooling techniques in the tweezers, which method should be preferred to achieve the highest ground state population? Why does Raman sideband (RSB) cooling work far better than any other process and is there a way to circumvent this experimentally tedious technique while still reaching comparable ground state population? During this presentation, I will address all these questions and discuss simulations that support the theoretical framework for Rubidium (Rb) and Lithium (Li) under realistic experimental conditions. Our model will also provide a unified framework to compare all sub-Doppler cooling methods used for a single atom in a tweezer and present a criterion to get the highest possible ground state population via each route.} - abstract.

% References
% Free-space
% Gray molasses potassium free-space \cite{salomon2014gray}
% $\Lambda$-enhanced GM of Li with D1 \cite{grier2013lambda}
% gray molasses sodium  \cite{colzi2016sub}
% gray molasses Cs \cite{boiron1996laser}
% Li6 D1 fray molasses Zaccanti group \cite{burchianti2014efficient}
% Cs D2 gray molasses 2018  \cite{hsiao2018lambda}
% 39 K , unnikrishan group.  \cite{nath2013quantum}

% Tweezer
% Regal \cite{brown2019gray}
% Gadway group \cite{huang2022gray}
% us \cite{blodgett2023imaging}
% ground state cooling paper RSB \cite{kaufman2012cooling}
% ground state cooling with RSB \cite{thompson2013coherence}
% \cite{kaufman2014two}
% energy distribution and cooling of single atom in tweezer   \cite{tuchendler2008energy}
% ni gruop, motional grounds state cooling outside LD regime  \cite{yu2018motional}
% Raman cooling imaging \cite{lester2014raman}
% Sr ground state cooling \cite{holzl2023motional}
% optical tweezer review Ni and Kuaffman \cite{kaufman2021quantum}
% Sr Endres \cite{cooper2018alkaline}
% Kaffman gruop
% Ytterbium Kauffman \cite{jenkins2022ytterbium}
% Yt narrow line cooling \cite{saskin2019narrow}

% Few body physics
% tweezer hopping \cite{young2022tweezer}
% jochim  \cite{bergschneider2018spin}
% pauli crystal jochim \cite{holten2021observation}


% Molecule
% Ni group, ground state \cite{zhang2022optical}
% prepartation heteronuclear in ground state, zhan group  \cite{wang2019preparation}
% lawrence 2019 tweezer array of molecules   \cite{anderegg2019optical}
% RSB of molecule \cite{lu2023raman}
% tarbutt theory for molecule sideband\cite{caldwell2020sideband}

% EIT cooling
% Blatt ground state with EIT  \cite{roos2000experimental}
% double EIT  \cite{evers2004double}
% Morigi  EIT cooling to ground state \cite{morigi2000ground}
% Morigi EIT cooling to ground state \cite{morigi2003cooling}
% Kurh group \cite{haller2015single}


% PG Theory
% Cohern Tnanou. Laser cooling below doppler limit   \cite{dalibard1989laser}
% PG cooling of ion theory quantum version \cite{wineland1992sisyphus}
% PG in LD regime for ions \cite{cirac1993laser}
% Theory for PG of ion, saem time as circa\cite{yoo1993polarization} 
% PG cooling exerpiemtn LD regime for ions, Schmidt-Kaler group  \cite{li2022robust}
% PG cooling study in dipole trap experiment Kurtsiefer gruop\cite{chin2017polarization}
% PG cooling in ions by Roos group \cite{joshi2020polarization}


% Based on free-space principles.

% PG cooling has used for atom in lattices, based on same principles. Doppler cooling in free-space limit, but LD regime, two distinct regimes.  For PG, GM,  what are the regimes. Diferent depedences.
% Recent new results in Li6 shows order of magnetidue improvement with the lightest atom using lambda - GM.  Does the position of the matter?  Does the polarization configuration matteR?  Any most importantly what are fundmaental limits to each of these schemes, can these schemes be improved?  What is the best strategy for imaging and cooling. 


% \Jon{Jon will write this section at end}
% \the\textwidth
% %Outline
% % history of cooling in LD regime
%     % RSB ?
%     %
% % history specficially of tweeezers
% % lattice cooling?
% % Unifying picture of cooling in LD regime - PG cooling, resolve unresolved sideband cooling, EIT, GM, lambda-enhanced GM, doppler, raman sideband cooling,  molecule cooling. 
% % This can't be a full review of cooling techniques. too much to cover.  Scope needs to be narorw - neutral atoms in tweezers.
% % Goals of the atoms in tweezers
%     % Rydberg
%     % Few-body physics
%     % Molecule assembly
%     % atomic clock
%     % latttice of atoms for quantum gas

% Cooling and imaging atoms in optical tweezers provide a new platform for Rydberg gates, deterministic molecule formation, and few-body and many-body Bose-Hubbard simulations. Rearrangement of tweezer results can produce defect-free lattices of atoms in 1D, 2D, and 3D. Cooling to the ground state is necessary for molecule formation and few-body physics. Temperature is also a limitation for gate fidelity due to the noise of interaction caused by thermal motion. The ground state in mK deep optical tweezers was first demonstrated using Raman sideband cooling.

% Two types of cooling are performed for atoms in tweezers. The recoil temperature for Cs is 200 nK and for the lightest alkali Li it is 3uK, which means only a few hundred photons can be scattered before loss. However, high NA objectives of ~0.6 only acquire a few percent of photons, meaning that to achieve 99$\%$ fidelity requires cooling during imaging. Currently, several types of cooling are performed during imaging: polarization gradient cooling, lambda-enhanced gray molasses, Raman sideband cooling, or single-photon sideband cooling. Recent evidence suggests that for alkali atoms, lambda-enhanced gray molasses provides 100x better imaging fidelity.

% For ground state preparation, only Raman sideband cooling is used. While the formalism has been developed for RSB, the conceptual pictures for PG and GM are still based on free-space models. Current theory models include Cohen-Ton for PG, Saloman and Weidemuller for GM, Thompson and Kaufman for RSB, and Endres with narrow-line cooling and Sisyphus cooling.

% % We have developed a formalism that applies to all cooling methods and shows that for PG and GM it provides more accurate temperature and imaging fidelity estimation and better scaling than free-space models. All schemes can be simplified by two main criteria: 1) A light shift that brings two adjacent states n and n-1 closer to resonance.

% Cooling and imaging atoms in optical tweezers a new platform for Rdyberg gates, deterministic molecule formation, and few-body and many-body Bose-Hubbard simulations.   Rearrangement tweezer results to get defect free lattices of atoms in 1D 2D and 3D.  Cooling to the ground state necessary for molecule formation, few-body physics, .  Temperature also is a limitation for gate fidelity to the noise of interaction cause by thermal motion.   Ground state in mK deep optical tweezer first demonstrated using Raman sideband cooling. 

% % Two types cooling performed for atoms in tweezers.  A recoil temperature for Cs is 200 nK or for the lightest alkali Li 3uK, means you can only scatter a few hundred photons before loss.  But high NA objectives of ~0.6 only acquire a few percent of photons, means that to get to 99$\%$ fidelity requires cooling during imaging.   Currently, several types of cooling are performed during imaging:   polarization gradient cooling, lambda enhanced gray molasses, and Raman sideband cooling, or single photon sideband cooling.   Lately evidence that for alkali atoms the lambda enhanced gray molasses is 100x better imaging fidelity. 

% % For ground state preparation, only Raman sidebande cooling.   While the formalism has been developed for RSB,  the conceptual pictures for PG and GM are still based on the free-space pictures.  - current theoretical models.   Cohen-Ton for PG.  Saloman and Weidemuller for GM.  Thompson and Kaufman for RSB.   Endres with narrow line cooling and sysphus cooling. linlin vs sigmaplus sigmaminus.

% We develop a formalism that applies to all cooling methods, and show that for PG and GM provide more accurate temperature and imaging fidelity estimation and better scaling than the free-space models.  Show the simple models. 
% -All schemes can be simplified by two main criteria:  1  A light shift that makes two adjacent n  and n-1 state closer to resonance, a coupling between them, and a dark and excited state within an atom. 

% % Summary of what we do:  Show how all the cooling l and show how all the cooling schemes are related to a single principle.  
% % -Estimate the coldest temperature and brightness of the different methods. 
% % The formalism also suggests some new strategies for colder cooling.  Include spilling.  Dark sideband cooling. 
% % -polarization-gradient (PG), gray molasses (GM), lambda-enhanced GM, single-photon and two-photon sideband cooling. 
% % Show a unified picture of cooling that captures...
% % -All schemes can be simplified by two main criteria:  1  A light shift that makes two adjacent n  and n-1 state closer to resonance, a coupling between them, and a dark and excited state within an atom. 


% While the formalism of Doppler cooling and Raman-sideband cooling have been worked out, we unite the resolved and unresolved Doppler cooling, PG, GM, $\Lambda$-GM, and EIT cooling in a simple framework using the LD expansion.  Show temperature limitations.  The picture also suggests new types of cooling schemes.  Strategies for tweezer experiments going forward.  




% \clearpage


% \begin{equation}
%     \frac{d \rho}{dt} = -i/\hbar [H, \rho ]  + \sum_i \frac{\Gamma}{2}  \mathcal{L}_C[ \rho] 
% \end{equation}
% with the Lindbladian 
% $\mathcal{L}_{\hat{C}}[\rho] =  \hat{C} \rho \hat{C}^\dag - \frac{1}{2} \left(\hat{C}^\dag \hat{C} \rho - \rho \hat{C}^\dag \hat{C} \right) $.  Spontaneous emission is modeled as a collapse operator $\hat{C} =  \sigma e^{\pm i k \hat{z}} $.

% This detuning is where the slope of scattering with velocity, and hence the damping, is largest. 
% Doppler cooling, also called optical molasses, cools the atom in both directions by including a counterpropagating laser, resulting in a damping force . The steady-state temperature is found by balancing the cooling from the damping and the heating from spontaneous emission.  It is limited by the excited state linewidth $T_\text{Doppler} = \hbar \Gamma/k_B $ and occurs at a laser detuning $\Delta = \omega_A - \omega_L = - \Gamma/2$. This detuning is where the slope of scattering with velocity, and hence the damping, is largest. 
% This simple model of cooling demonstrates an important principle of laser cooling: the final temperature is limited by how well the second state can be resolved.  Narrower transitions, like those found in alkaline-earth atoms, or narrow transitions in alkali atoms, results in lower temperature. 

% Cooling in free-space is typically treated with a semi-classical model, where the atom position and electric field are classical and the emitter is quantum.  This paper will focus on neutral atoms in a 1D harmonic potential $V(z) = 1/2 m \nu^2 z^2 $. When the scattering rate is comparable or lower than the oscillating frequency, only a single laser beam is required to cool. As the atom oscillates in the trap at frequency $\nu$, the phase in the frame of the atom will modulate leading to two sidebands $\omega_L \pm \nu$ on the laser in the frame of the atom. If the laser is detuned below the transition frequency by the trapping frequency $\nu$, then the higher sideband is resonant and scatters more photons. The sponteneously emitted photons at frequency $\omega$ take away the atom's kinetic energy.  

% Classically, this can be viewed as the atomic response function filtering out the lower frequency sideband, leading to amplitude modulation of the light in the frame of the atom.  This modulates the dipole force exerted by the light on the atom, and the component of this modulation out of phase with the atom's oscillation dampens the energy of the atoms motion. Again, the damping is countered by the recoil heating associated with the scattering of photons resulting in a steady state temperature. 

% Two distinct regimes of cooling arise in a harmonic trap. The unresolved sideband cooling regime is when the harmonic frequency is smaller than the transition linewidth $\nu < \Gamma$.  The final temperature converges to free-space Doppler temperature for small $\nu$. The other regime is where the trapping frequency is comparable or larger than the transition linewith  $\nu > \Gamma$, where then the carrier and lower sideband are off-resonant resulting in less overall scattering.  In the resolved-sideband regime, the steady state temperature can be much lower than the Doppler temperature.   %This result demonstrates the second principle of laser cooling: the temperature scales with the overall scattering rate. 

% The semi-classical model breaks down when the trapping frequency is comparable to the photon recoil energy $E_R = (\hbar k)^2/(2 m) $. Then the quantizization of atoms harmonic motion is important.  The position must be treated quantum mechanically.  





% \end{document}
